# Supplementary material for: On the number of principal components in high dimensions
Source: arXiv:1708.04981 ancillary file (2017-08-16)
Supplement: Supplementary file 1 [file NPCHDSupplement.pdf]

*Biometrika* (2017), **xx**, x, *pp*. 1–25
© 2007 Biometrika Trust
*Printed in Great Britain*

# Supplementary material for "On the number of principal components in high dimensions"

BY SUNGKYU JUNG
*Department of Statistics, University of Pittsburgh, Pittsburgh, Pennsylvania, 15260, U.S.A.*
sungkyu@pitt.edu

MYUNG HEE LEE
*Center for Global Health, Department of Medicine, Weill Cornell Medicine, New York, New York, 10065, U.S.A.*
myl2003@med.cornell.edu

AND JEONGYOUN AHN
*Department of Statistics, University of Georgia, Athens, Georgia, 30602, U.S.A.*
jyahn@uga.edu

## S1. ASYMPTOTIC NORMALITY OF $S_D$

The asymptotic normality of the elements of $S_D$ in Theorem 1 and the rate of convergence are main technical tools we use.

### S1·1. *Proof of Theorem 1*

The convergence in probability of $S_D$ to $W_1 W_1^{\mathrm{T}} + \tau^2 I_n$ is obtained by Theorem 2 of Jung et al. (2012). Here, we give a proof of the following:

$$\sqrt{d}\left(s_{jj} - \sum_{i=1}^{m} \sigma_i^2 z_{ij}^2 - \tau^2\right) \longrightarrow N(0, \upsilon_D^2), \quad \text{for } 1 \le j \le n, \tag{S1.1}$$

$$\sqrt{d}\left(s_{jk} - \sum_{i=1}^{m} \sigma_i^2 z_{ij} z_{ik}\right) \longrightarrow N(0, \upsilon_O^2), \quad \text{for } 1 \le j \ne k \le n, \tag{S1.2}$$

in distribution as $d \to \infty$. Note that the $(j,k)$th element of $S_D$ is $s_{jk} = \sum_{i=1}^{m} \sigma_i^2 z_{ij} z_{ik} + \frac{1}{d}\sum_{i=m+1}^{d} \lambda_i z_{ij} z_{ik}$.

We first show (S1.1). For a fixed $j = 1, \ldots, n$, let $Y_i = \lambda_i(z_{ij}^2 - 1)$. Then $E(Y_i) = 0$ and $s_d^2 := \mathrm{var}(\sum_{i=m+1}^{d} Y_i) = \sum_{i=m+1}^{d} \lambda_i^2 \mathrm{var}(z_{ij}^2)$. Let $\delta \in (0, 1]$ satisfy Condition 2, and denote $A_d = \sum_{i=m+1}^{d} E(|Y_i|^{2+\delta})/(s_d^{2+\delta})$ for each $d$. Denote $\tilde{z}_i = |z_{ij}^2 - 1|$ for simplicity. By an application of Hölder's inequality and by Condition 3, there exists a finite $B$ such that for any $i$,

$$E(\tilde{z}_i^{2+\delta}) \le \{E(\tilde{z}_i^3)\}^{(2+\delta)/3} \le B < \infty.$$

This leads to

$$\sum_{i=m+1}^{d} E(|Y_i|^{2+\delta}) = \sum_{i=m+1}^{d} \lambda_i^{2+\delta} E(\tilde{z}_i^{2+\delta}) \leq B \sum_{i=m+1}^{d} \lambda_i^{2+\delta}, \text{ for any } d. \tag{S1.3}$$

Since $\mathrm{var}(z_{ij}^2)$ are uniformly bounded below, we have

$$s_d^2 = \sum_{i=m+1}^{d} \lambda_i^2 \mathrm{var}(z_{ij}^2) \geq \epsilon \sum_{i=m+1}^{d} \lambda_i^2, \text{ for any } d. \tag{S1.4}$$

Combining (S1.3)–(S1.4) together with Condition 2, the Lyapunov condition is satisfied:

$$A_d = \frac{\sum_{i=m+1}^{d} E(|Y_i|^{2+\delta})}{s_d^{2+\delta}} \leq \frac{B \sum_{i=m+1}^{d} \lambda_i^{2+\delta}}{\epsilon^{1+\delta/2} (\sum_{i=m+1}^{d} \lambda_i^2)^{1+\delta/2}} \to 0, \text{ as } d \to \infty, \tag{S1.5}$$

which in turn leads that

$$s_d^{-1} \sum_{i=m+1}^{d} Y_i = \left\{ \sum_{i=m+1}^{d} \lambda_i^2 \mathrm{var}(z_{ij}^2) \right\}^{-1/2} \sum_{i=m+1}^{d} \lambda_i (z_{ij}^2 - 1) \longrightarrow N(0,1)$$

in distribution as $d \to \infty$. Since $s_d^2 \asymp d$, (S1.1) is proved.

Next, to show (S1.2), define $Y_i = \lambda_i z_{ij} z_{ik}$, for any given pair $(j,k)$, where $1 \leq j \neq k \leq n$. Since $z_{ij}$ and $z_{ik}$ are independent for all $i$, we have $E(Y_i) = 0$ and $s_d^2 := \mathrm{var}(\sum_{i=m+1}^{d} Y_i) = \sum_{i=m+1}^{d} \lambda_i^2$. Similar to the arguments used in (S1.3)–(S1.5), there exists a finite $B_1$ such that

$$\frac{\sum_{i=m+1}^{d} E(|Y_i|^{2+\delta})}{s_d^{2+\delta}} \leq \frac{B_1 \sum_{i=m+1}^{d} \lambda_i^{2+\delta}}{(\sum_{i=m+1}^{d} \lambda_i^2)^{1+\delta/2}} \to 0,$$

in probability as $d \to \infty$. Thus, again by Lyapunov central limit theorem, we have

$$\left( \sum_{i=m+1}^{d} \lambda_i^2 \right)^{-1/2} \sum_{i=m+1}^{d} \lambda_i z_{ij} z_{ik} \to N(0,1)$$

in distribution as $d \to \infty$, which in turn leads to (S1.2).

### S1·2. *Convergence for eigenvalue decomposition of $S_D$*

The findings in Theorem 1 are now used to establish a rate of convergence for the eigenvalues and eigenvectors of $S_D$, shown in Lemma S1.1 below. The eigenvectors of $S_D$ are proportional to the vector whose elements are the sample principal component scores. Lemma S1.1 will be used in establishing a convergence of the sample principal component directions, through the well-known relationship between the eigen-decomposition and singular value decomposition; $\mathcal{X}^{\mathrm{T}} = n^{1/2} \widehat{U} \widehat{\Lambda}^{1/2} \widehat{V}^{\mathrm{T}} = n^{1/2} \sum_{i=1}^{n} \hat{\lambda}_i^{1/2} \hat{u}_i \hat{v}_i^{\mathrm{T}}$, where $(\hat{\lambda}_i, \hat{u}_i)$ and $(\hat{\lambda}_i, \hat{v}_i)$ are the eigenvalue-eigenvector pairs of $S_d$ and $dn^{-1} S_D$, respectively. Let $S_0 = W_1 W_1^{\mathrm{T}} + \tau^2 I_n$. See (11) in the main article for the definition of $W_1$.

LEMMA S1.1. *Assume the $m$-factor model under Conditions 1–3. Let $n > m \geq 0$ be fixed and $d \to \infty$. The eigenvalues and eigenvectors of $S_D$ converge to those of $S_0$ in probability, with*

*convergence rate of $\sqrt{d}$. Specifically,*

$$\lambda_i(S_D) - \lambda_i(S_0) = O_p(d^{-1/2}), \quad \textit{for } i = 1, \ldots, n, \tag{S1.6}$$

$$\|v_i(S_D) - v_i(S_0)\|_2 = O_p(d^{-1/2}), \quad \textit{for } i = 1, \ldots, m. \tag{S1.7}$$

*Proof.* By Theorem 1, we can write $S_D = S_0 + E_d$, where $E_d$ satisfies $\|E_d\|_2 = O_p(d^{-1/2})$, and the largest and smallest eigenvalues of $E_d$ are both real and $O_p(d^{-1/2})$. Writing $\lambda_i(S_D) = \lambda_i(S_0 + E_d)$, Weyl's inequality gives $\lambda_i(S_0) + \lambda_n(E_d) \leq \lambda_i(S_0 + E_d) \leq \lambda_i(S_0) + \lambda_1(E_d)$, for all $i = 1, \ldots, n$, which proves (S1.6).

To show (S1.7), we use the following lemma (a proof of which is given later in this section).

LEMMA S1.2. *Let $A$ and $E$ be $n \times n$ real symmetric matrices. Let $Q = [q : Q_2]$ be a $n \times n$ orthonormal matrix with $q$ satisfying $Aq = \lambda q$ for some eigenvalue $\lambda$ of $A$. Write $Q^T AQ = Diag\{\lambda, \Lambda_o\}$. If $\delta = \min\{|\lambda - \lambda(\Lambda_o)|\} > 0$, where $\lambda(\Lambda_o)$ denotes the set of all eigenvalues of $\Lambda_o$, and $\|E\|_2 \leq \delta/5$, then*

*(i) there exists $p \in \mathbb{R}^{n-1}$ with $\|p\|_2 \leq \frac{4}{\delta}\|E\|_2$ such that $\hat{q} = (q + Q_2 p)(1 + p^T p)^{-1/2}$ is an eigenvector of $A + E$.*
*(ii) Additionally if $\lambda$ is the $r$th largest eigenvalue of $A$ with multiplicity 1, then the eigenvalue of $A + E$ corresponding to $\hat{q}$ is the $r$th largest eigenvalue of $A + E$.*

In Lemma S1.2 the unit vector $q$ is the eigenvector corresponding to an eigenvalue $\lambda$ of $A$. The lemma provides an upper bound on $\|q - \hat{q}\|_2$. The statement (ii) assures that we compare the right pair, that is, if $q$ is the $r$th eigenvector of $A$, then $\hat{q}$ is the $r$th eigenvector of $A + E$.

Now, let $S_0$ and $E_d$ be $A$ and $E$ of Lemma S1.2. For $i \leq m$, let $q := v_i(S_0)$ so that $\lambda := \lambda_i(S_0)$ has non-zero spacing $\delta > 0$. Since $\|E_d\|_2 = O_p(d^{-1/2})$, the condition $\|E_d\|_2 \leq \delta/5$ is satisfied for a sufficiently large $d$. Then by Lemma S1.2, there exists $p \in \mathbb{R}^{n-1}$ such that $v_i(S_0 + E_d) = (q + Q_2 p)(1 + p^{\mathrm{T}} p)^{-1/2}$ and

$$\|p\|_2 \leq \frac{4}{\delta}\|E\|_2 = O_p(d^{-1/2}). \tag{S1.8}$$

Combining the equation

$$\begin{aligned} \|v_i(S_D) - v_i(S_0)\|_2^2 = \|q - \hat{q}\|_2^2 = 2(1 - q^{\mathrm{T}}\hat{q}) &= 2\left\{1 - (1 + p^{\mathrm{T}} p)^{-1/2}\right\} \\ &= 2\left[1 - \left\{1 - \|p\|_2^2/2 + O_p(\|p\|_2^4)\right\}\right] \\ &= \|p\|_2^2 + O_p(\|p\|_2^4), \end{aligned}$$

and (S1.8) gives (S1.7). □

*Proof of Lemma S*1.2. A proof of (i) can be obtained by Theorem 8.1.10 of Golub & Van Loan (1996).

For (ii), let $\hat{\lambda}$ be such that

$$(A + E)\hat{q} = \hat{\lambda}\hat{q}. \tag{S1.9}$$

It is enough to show that $\hat{\lambda} \in (\lambda_{r+1}(A + E), \lambda_{r-1}(A + E))$.

Pre-multiplying $q^{\mathrm{T}}$ to (S1.9) gives $q^{\mathrm{T}} A\hat{q} + q^{\mathrm{T}} E\hat{q} = \hat{\lambda} q^{\mathrm{T}}\hat{q}$. Since $A$ is symmetric, we have $q^{\mathrm{T}} A = (Aq)^{\mathrm{T}} = \lambda q^{\mathrm{T}}$; $|q^{\mathrm{T}} E\hat{q}| \leq \|q\|_2\|E\|_2\|\hat{q}\|_2 = \|E\|_2$; $q^{\mathrm{T}}\hat{q} = (1 + p^{\mathrm{T}} p)^{-1/2} = (1 + \|p\|_2^2)^{1/2} \geq 1/\sqrt{2}$, since $\|p\|_2 \leq 1$. By writing $\lambda = \lambda_r(A)$, these facts together lead to the fol-

lowing:

$$\lambda_r(A) - \sqrt{2}\|E\|_2 \leq \hat{\lambda}, \tag{S1.10}$$

$$\lambda_r(A) + \sqrt{2}\|E\|_2 \geq \hat{\lambda}. \tag{S1.11}$$

By Weyl's inequality, we have

$$\lambda_{r+1}(A+E) \leq \lambda_{r+1}(A) + \|E\|_2, \tag{S1.12}$$

$$\lambda_{r-1}(A+E) \geq \lambda_{r-1}(A) - \|E\|_2. \tag{S1.13}$$

Combining (S1.10) and (S1.12) gives

$$\begin{aligned}\hat{\lambda} - \lambda_{r+1}(A+E) &\geq \lambda_r(A) - \lambda_{r+1}(A) - (1+\sqrt{2})\|E\|_2 \\ &\geq \delta - (1+\sqrt{2})\|E\|_2 \\ &\geq (1 - \frac{1+\sqrt{2}}{5})\delta > 0,\end{aligned}$$

where the second inequality is from the definition of $\delta$ and the last inequality is by the assumption. Similarly, combining (S1.11) and (S1.13) gives $\lambda_{r-1}(A+E) - \hat{\lambda} > 0$. □

## S2. LIMITING BEHAVIORS OF SAMPLE PRINCIPAL COMPONENTS

In Section S2·1, Theorem S2.1 provides a $d$-asymptotic behaviors of the PC estimates, and Lemma S2.1 generalizes Theorem 1 of Hellton & Thoresen (2017). In Section S2·2, a proof of Theorem 4 is given.

### S2·1. *d-asymptotic behaviors of the PCA*

THEOREM S2.1. *Assume the $m$-factor model under Conditions 1–3 and let $n > m \geq 0$ be fixed and $d \to \infty$. Let $\gamma_k \in [0, 0.5)$ so that $\lambda_k \asymp d^{\gamma_k}$. Conditional to $W_1$, (i) the sample principal component variances converge in probability as $d \to \infty$;*

$$d^{-1}n\hat{\lambda}_i = \begin{cases} \lambda_i(W_1W_1^{\mathrm{T}}) + \tau^2 + O_p(d^{-1/2}), & i = 1,\ldots,m; \\ \tau^2 + O_p(d^{-1/2}), & i = m+1,\ldots,n. \end{cases} \tag{S2.1}$$

*(ii) The inner product between sample and population PC directions converges in probability as $d \to \infty$;*

$$\hat{u}_i^{\mathrm{T}}u_j = \begin{cases} \frac{v_{ij}(W_1W_1^{\mathrm{T}})}{\sqrt{1+\tau^2/\lambda_i(W_1W_1^{\mathrm{T}})}} + O_p(d^{-1/2}), & i,j = 1,\ldots,m; \\ O_p(d^{-1/2}), & i > m, j \leq m; \\ O_p(d^{-(1-\gamma_k)/2}), & j > m. \end{cases} \tag{S2.2}$$

*Proof.* (i) Since $d^{-1}nS_d = d^{-1}\mathcal{X}^{\mathrm{T}}\mathcal{X}$ shares the same non-zero eigenvalues with $d^{-1}\mathcal{X}\mathcal{X}^{\mathrm{T}} = S_D$, we have, for $1 \leq i \leq m$, $d^{-1}n\hat{\lambda}_i = \lambda_i(S_D) = \lambda_i(S_0) + O_p(d^{-1/2})$ by Lemma S1.1. Observing $\lambda_i(S_0) = \lambda_i(W_1^{\mathrm{T}}W_1) + \tau^2 = \lambda_i(W_1W_1^{\mathrm{T}}) + \tau^2$ and that $W_1W_1^{\mathrm{T}}$ is rank $m$ give (S2.1).

(ii) It is easy to see that, for $i = 1,\ldots,n$, $\hat{u}_i = (n\hat{\lambda}_i)^{-1/2}\mathcal{X}^{\mathrm{T}}\hat{v}_i$. By writing $\mathcal{X}^{\mathrm{T}} = U\Lambda^{1/2}Z$, the inner product $\hat{u}_i^{\mathrm{T}}u_j$ becomes, for $i = 1,\ldots,n$,

$$\hat{u}_i^{\mathrm{T}}u_j = (n\hat{\lambda}_i)^{-1/2}u_j^{\mathrm{T}}\mathcal{X}^{\mathrm{T}}\hat{v}_i = \begin{cases} (d^{-1}n\hat{\lambda}_i)^{-1/2}\sigma_j(z_{j1},\ldots,z_{jn})\hat{v}_i, & j = 1,\ldots,m; \\ (d^{-1}n\hat{\lambda}_i)^{-1/2}(d^{-1}\lambda_j)^{1/2}(z_{j1},\ldots,z_{jn})\hat{v}_i, & j > m. \end{cases} \tag{S2.3}$$

Here, $(z_{j1},\ldots,z_{jn})$ denotes the row vector consisting of entries $z_{j1},\ldots,z_{jn}$. We show (S2.2) for three different cases of $i$ and $j$, using (S2.3).

**Case 1** ($i, j \le m$)**:** By Lemma S1.1, $\hat{v}_i = v_i(S_D) = v_i(S_0) + O_p(d^{-1/2})$, and by (S2.1) $d^{-1}n\hat{\lambda}_i = \lambda_i(W_1W_1^{\mathrm{T}}) + \tau^2 + O_p(d^{-1/2})$. Since

$$\sigma_j(z_{j1}, \ldots, z_{jn})v_i(S_0) = \sqrt{\lambda_i(W_1W_1^{\mathrm{T}})}v_{ij}(W_1W_1^{\mathrm{T}}),$$

(S2.2) follows for this case.

**Case 2** ($i > m, j \le m$)**:** In this case, we have $d^{-1}n\hat{\lambda}_i = \tau^2 + O_p(d^{-1/2})$ from Theorem S2.1. (S2.2) is obtained by combining (S2.3) and the following claim:

$$\sigma_j(z_{j1}, \ldots, z_{jn})\hat{v}_i = O_p(d^{-1/2}). \tag{S2.4}$$

To show (S2.4), first observe that $\sigma_j(z_{j1}, \ldots, z_{jn})$ is the $j$th row of $W_1$, which is a linear combination of the first $m$ eigenvectors of $W_1^{\mathrm{T}}W_1$. Specifically, there exist $a_{kj} \in \mathbb{R}$, $(k = 1, \ldots, m, j = 1, \ldots, n)$ such that

$$\sigma_j(z_{j1}, \ldots, z_{jn})^{\mathrm{T}} = \sum_{k=1}^{m} a_{kj}v_k(W_1^{\mathrm{T}}W_1) = \sum_{k=1}^{m} a_{kj}v_k(S_0). \tag{S2.5}$$

By Lemma S1.1, we can write $v_k(S_0) = \hat{v}_k + O_p(d^{-1/2})$, for $k \le m$, and together with (S2.5), we have $\sigma_j(z_{j1}, \ldots, z_{jn})\hat{v}_i = \sum_{k=1}^{m} a_{kj}(\hat{v}_k^{\mathrm{T}} + O_p(d^{-1/2}))\hat{v}_i = O_p(d^{-1/2})$ as required. Here, we use the fact $\hat{v}_k^{\mathrm{T}}\hat{v}_i = 0$ for $i \ne k$.

**Case 3** ($j > m$)**:** The result is obtained by noting that the first term $(d^{-1}n\hat{\lambda}_i)^{-1/2}(d^{-1}\lambda_j)^{1/2}$ of (S2.3) is $O_p(d^{-(1-\gamma_k)/2})$, while the later term is $O_p(1)$. □

The following lemma, generalizing Theorem 1 of Hellton & Thoresen (2017), characterizes the ratio of the sample standardized score, defined by $\hat{z}_{kj} = (\hat{\lambda}_k)^{-1/2}\hat{w}_{kj}$, to the true score $z_{kj}$. We use the notation $\mathcal{W} = W_1W_1^{\mathrm{T}}$, which is an $m \times m$ symmetric positive definite matrix.

LEMMA S2.1. *Let $k \le m$. Under the assumptions of Theorem 4, $\hat{z}_{kj}/z_{kj}$ is asymptotically decomposed into a common factor $R_k'$ and an idiosyncratic error $\epsilon_{kj}'$, as $d \to \infty$, Here, $R_k'$ and $\epsilon_{kj}'$ are defined at (S2.7) below.*

*Proof.* Note that $\hat{z}_k = (\hat{z}_{k1}, \ldots, \hat{z}_{kn})^{\mathrm{T}} = \sqrt{n}\hat{v}_k$, where $\hat{v}_k$ is the $k$th eigenvector of $S_D$. Since $(\hat{v}_k)_j = v_{kj}(S_0) + O_p(d^{-1/2})$ (by Lemma S1.1), we obtain

$$\frac{\hat{z}_{kj}}{z_{kj}} = \frac{\sqrt{n}(\hat{v}_k)_j}{z_{kj}} = \frac{\sqrt{n}v_{kj}(S_0)}{z_{kj}} + O_p(d^{-1/2}). \tag{S2.6}$$

Rearranging the terms in

$$v_{kj}(S_0) = \lambda_k^{-1/2}(\mathcal{W})(\sigma_1 z_{1j}, \ldots, \sigma_m z_{mj})v_k(\mathcal{W}) = \lambda_k^{-1/2}(\mathcal{W})\sum_{i=1}^{m}\sigma_i z_{ij}v_{ki}(\mathcal{W})$$

leads to $\frac{\hat{z}_{kj}}{z_{kj}} = R_k' + \epsilon_{kj}' + O_p(d^{-1/2})$, where

$$R_k' = \sqrt{\frac{n\sigma_k^2}{\lambda_k(\mathcal{W})}}v_{kk}(\mathcal{W}), \quad \epsilon_{kj}' = \sqrt{\frac{n\sigma_k^2}{\lambda_k(\mathcal{W})}}\sum_{1\le i\le m, i\ne k}\frac{\sigma_i z_{ij}}{\sigma_k z_{kj}}v_{ki}(\mathcal{W}). \quad \square \tag{S2.7}$$

### S2·2. *Proof of Theorem 4*

We continue to use the notation $\mathcal{W} = W_1W_1^{\mathrm{T}}$.

(i) Note that $\frac{\hat{w}_{kj}}{w_{kj}} = \sqrt{\frac{\hat{\lambda}_k}{\sigma_k^2 d}} \frac{\hat{z}_{kj}}{z_{kj}}$. By Theorem S2.1, the first term is

$$\sqrt{\frac{\hat{\lambda}_k}{\sigma_k^2 d}} = \sqrt{\frac{\lambda_k(\mathcal{W}) + \tau^2}{n\sigma_k^2}} + O_p(d^{-1/2}) = \rho_k \sqrt{\frac{\lambda_k(\mathcal{W})}{n\sigma_k^2}} + O_p(d^{-1/2}), \tag{S2.8}$$

where $\rho_k$ is defined in the statement of Theorem 4. Combining (S2.8) with (S2.6)-(S2.7) in the proof of Lemma S2.1 shows that

$$\frac{\hat{w}_{kj}}{w_{kj}} = \rho_k v_{kk}(W_1 W_1^{\mathrm{T}}) + \varepsilon_{kj} + O_p(d^{-1/4}) \quad (j = 1, \ldots, n),$$

as desired.

For a proof of (13), write $\widehat{W}_1^{\mathrm{T}} = (\hat{w}_1, \ldots, \hat{w}_m)$, where

$$\hat{w}_i = \sqrt{\frac{n}{d}} \hat{\lambda}_i \hat{v}_i = \sqrt{\lambda_i(S_0)} v_i(S_0) + O_p(d^{-1/2}). \tag{S2.9}$$

Let $W_1^{\mathrm{T}} = U_W D_W V_W^{\mathrm{T}}$ be the singular value decomposition of order $m$ for $W_1$. From $S_0 - \tau^2 I_n = W_1^{\mathrm{T}} W_1 = U_W D_W^2 U_W^{\mathrm{T}}$, we have

$$U_W = [v_1(S_0), \ldots, v_m(S_0)]. \tag{S2.10}$$

Likewise, from $\mathcal{W} = W_1 W_1^{\mathrm{T}} = V_W D_W^2 V_W^{\mathrm{T}}$, $D_W = \mathrm{diag}\{\sqrt{\lambda_1(\mathcal{W})}, \ldots, \sqrt{\lambda_m(\mathcal{W})}\}$ and thus $V_W = (v_1(\mathcal{W}), \ldots, v_m(\mathcal{W}))$, consisting of the eigenvectors of $\mathcal{W}$.

From (S2.9) and (S2.10), $\widehat{W}_1^{\mathrm{T}}$ converges to

$$\begin{aligned} &U_W \mathrm{diag}\{\sqrt{\lambda_1(S_0)}, \ldots, \sqrt{\lambda_m(S_0)}\} \\ &\quad = U_W D_W V_W^{\mathrm{T}} V_W D_W^{-1} \mathrm{diag}\{\sqrt{\lambda_1(\mathcal{W}) + \tau^2}, \ldots, \sqrt{\lambda_m(\mathcal{W}) + \tau^2}\} \\ &\quad = W_1^{\mathrm{T}} V_W \mathrm{diag}\{\sqrt{1 + \tau^2/\lambda_1(\mathcal{W})}, \ldots, \sqrt{1 + \tau^2/\lambda_m(\mathcal{W})}\}, \end{aligned}$$

in probability as $d \to \infty$, which proves (13).

Part (ii) is obtained by noting that $d^{-1}\hat{w}_{ki}^2 = d^{-1} n \hat{\lambda}_k (\hat{v}_k)_i^2 \to \tau^2 (v_{ki}(S_0))^2$ in probability as $d \to \infty$, and that $w_{ki} = \lambda_k z_{ki} = O_p(d^{\gamma_k})$. The last result is obtained by the constraint $\sum_{i=1}^n (v_{ki}(S_0))^2 = 1$.

## S3. PROOFS OF MAIN RESULTS

### S3·1. *A technical lemma*

We make use of the following lemma in the proof of Corollary 1.

LEMMA S3.1. *The sum of independent right-skewed random variables is also right-skewed. In particular, Let $X_1, \ldots, X_m$ be a collection of independent random variables satisfying $E(X_i - E(X_i))^3 > 0$ for all $i = 1, \ldots, m$. Then for $T = \sum_{i=1}^m a_i X_i$, where $a_i > 0$, $E(T - E(T))^3 > 0$.*

*Proof.* Let $m = 2$. Let $Y_i = X_i - E(X_i)$, $i = 1, 2$. Then $E(T - E(T))^3 = E(a_1 Y_1 + a_2 Y_2)^3 = a_1^3 E(Y_1^3) + a_2^3 E(Y_2^3) > 0$. Other cases of $m > 2$ are obtained by induction. □

### S3·2. *Proof of Corollary 1*

Write $\frac{1}{d}\sum_{i=m+1}^{d} w_{ij}^2 = s_{jj} - \sum_{i=1}^{m} \sigma_i^2 z_{ij}^2$. Then Theorem 1 gives

$$\sqrt{d}\Big(\frac{1}{d}\sum_{i=m+1}^{d} w_{ij}^2 - \tau^2\Big) \to N(0, \upsilon_D^2), \text{ in distribution as } d \to \infty. \quad \text{(S3.1)}$$

For $k \geq m$, we have $\tilde{R}_j(k) = \frac{1}{d}\sum_{i=m+1}^{d} w_{ij}^2 - \frac{1}{d}\sum_{i=k+1}^{m} w_{ij}^2$, and $\frac{1}{d}\sum_{i=k+1}^{m} w_{ij}^2 = O(d^{-1})$. Then, (S3.1) yields the asymptotic normality of $\tilde{R}_j(k)$;

$$\sqrt{d}(\tilde{R}_j(k) - \tau^2) \to N(0, \upsilon_D^2), \text{ in distribution as } d \to \infty. \quad \text{(S3.2)}$$

For $k < m$, we have $\tilde{R}_j(k) = \sum_{i=k+1}^{m} \sigma_i^2 z_{ij}^2 + \frac{1}{d}\sum_{i=m+1}^{d} w_{ij}^2$, which converges to $\sum_{i=k+1}^{m} \sigma_i^2 z_{ij}^2 + \tau^2$, conditioned on $z_{ij}$, $i \leq m$, for large $d$. Since each $z_{ij}^2$ is right-skewed, the sum, $\tilde{R}_j(k)$, is also right-skewed by Lemma S3.1.

### S3·3. *Proof of Theorem 2*

The case (i), where $m = 0$, is obtained by an application of Corollary 1. For any pair $(j, \ell)$ of sample indices such that $j \neq \ell$, choose $n > \max\{j, \ell\}$. Since $R_j(0) = \tilde{R}_j(0)$, Corollary 1 shows that the limiting distribution of $R_j(0)$ (as $d \to \infty$) is a normal distribution. Since $R_j(0)$ is a function of the $j$th observation $X_j$ only, taking the additional limit, $n \to \infty$, does not change the limiting distribution of $R_j(0)$. Finally, since for any $d$ and $n$, $R_j(0)$ does not depend on $X_\ell$ (and vice versa), $R_j(0)$ and $R_\ell(0)$ are independent.

Case (ii). It can be seen from (S3.2) in the proof of Corollary 1 that $\tilde{R}_j(m) = \tau^2 + O_p(d^{-1/2})$. As defined in (12) in the main article, let $a_j(m) = R_j(m) - \tilde{R}_j(m) = \frac{1}{d}\sum_{i=1}^{m}(w_{ij}^2 - \hat{w}_{ij}^2)$. Write $w_j = (w_{1j}, \ldots, w_{mj})^{\mathrm{T}}$. We use Theorem 4(i) to express $a_j(m)$ as $a_j(m) = w_j^{\mathrm{T}} w_j - w_j^{\mathrm{T}} R S^2 R^{\mathrm{T}} w_j + O_p(d^{-1/2})$, where

$$\begin{aligned} w_j^{\mathrm{T}} w_j - w_j^{\mathrm{T}} R S^2 R^{\mathrm{T}} w_j &= w_j^{\mathrm{T}} R \left(I_m - S^2\right) R^{\mathrm{T}} w_j \\ &= -\tau^2 w_j^{\mathrm{T}} R[\mathrm{diag}(1/\lambda_1(W_1 W_1^{\mathrm{T}}), \ldots, 1/\lambda_m(W_1 W_1^{\mathrm{T}}))] R^{\mathrm{T}} w_j \\ &= -\tau^2 w_j^{\mathrm{T}} (W_1 W_1^{\mathrm{T}})^{-1} w_j. \end{aligned}$$

Here, $\mathrm{diag}(l_1, \ldots, l_m)$ denotes the $m \times m$ diagonal matrix whose $i$th diagonal element is given by $l_i$ $(i = 1, \ldots, m)$. Simply put, $a_j(m) = -\tau^2 w_j^{\mathrm{T}} (W_1 W_1^{\mathrm{T}})^{-1} w_j + O_p(d^{-1/2})$. Thus, for any $n$, we have

$$R_j(m) = \tau^2 - \tau^2 w_j^{\mathrm{T}} (W_1 W_1^{\mathrm{T}})^{-1} w_j + O_p(d^{-1/2}).$$

We now approximate the $m \times m$ matrix $n^{-1} W_1 W_1'$ by its expectation $\Sigma_{W_1} = \mathrm{diag}(\sigma_1^2, \ldots, \sigma_m^2)$, by taking the limit $n \to \infty$. Since $n^{-1} W_1 W_1^{\mathrm{T}} - \Sigma_{W_1} = O_p(n^{-1/2})$, we use a classical result on matrix inversion error (Demmel, 1992); $(\frac{1}{n} W_1 W_1^{\mathrm{T}})^{-1} = \Sigma_{W_1}^{-1} + O_p(n^{-1/2})$. Therefore, we have

$$\begin{aligned} -\tau^2 w_j^{\mathrm{T}} (W_1 W_1^{\mathrm{T}})^{-1} w_j &= -\frac{\tau^2}{n} w_j^{\mathrm{T}} (n^{-1} W_1 W_1^{\mathrm{T}})^{-1} w_j \\ &= -\frac{\tau^2}{n} w_j^{\mathrm{T}} [\Sigma_{W_1}^{-1} + O_p(n^{-1/2})] w_j \\ &= -\frac{\tau^2}{n} \sum_{i=1}^{m} z_{ij}^2 + O_p(n^{-3/2}). \end{aligned}$$

Rearranging the terms gives

$$n(R_j(m) - \tau^2) = A_j(m) + O_p(n^{-1/2}) + O_p(n/d), \tag{S3.3}$$

and $n(R_j(m) - \tau^2) \to A_j(m)$ in probability, as $d \to \infty$ and $n \to \infty$. Lemma S3.1 ensures that $A_j(m) = -\tau^2 \sum_{i=1}^m z_{ij}^2$ is left-skewed. Since $\{(z_{1j}, \ldots, z_{mj}) : j = 1, 2, \ldots\}$ is an independent and identically distributed (i.i.d) sequence of random variables (by Condition 3), $\{A_j(m) : j = 1, 2, \ldots\}$ is also i.i.d.

Case (iii). We begin by writing $R_j(k)$ as $R_j(k) = \tilde{R}_j(k) + a_j(k)$, where

$$\tilde{R}_j(k) = \sum_{i=k+1}^{m} \sigma_i^2 z_{ij}^2 + \tau^2 + O_p(d^{-\frac{1}{2}}) \tag{S3.4}$$

$$a_j(k) = \frac{1}{d}\sum_{i=1}^{k}(w_{ij}^2 - \hat{w}_{ij}^2) = \sum_{i=1}^{k} \sigma_i^2 z_{ij}^2 (1 - \frac{\hat{w}_{ij}^2}{w_{ij}^2}). \tag{S3.5}$$

We simplify the ratio $\hat{w}_{ij}^2 / w_{ij}^2$ by taking the limit $d \to \infty$ according to Theorem 4(i). Furthermore, we use a classical results on the asymptotic distributions of principal component directions and variances for the $m \times m$ matrix $\frac{1}{n} W_1 W_1^{\mathrm{T}}$ (given by the asymptotic direction $n \to \infty$). In particular, from Muirhead (1982), for any $i, \kappa = 1, \ldots, m$ and $i \neq \kappa$,

$$v_{ii}(W_1 W_1^{\mathrm{T}}) = 1 + O_p(n^{-1/2}),$$
$$v_{i\kappa}(W_1 W_1^{\mathrm{T}}) = O_p(n^{-1/2}),$$
$$\lambda_i(\frac{1}{n} W_1 W_1^{\mathrm{T}}) = 1 + O_p(n^{-1/2}).$$

Then $\rho_i = \{1 + \tau^2/\lambda_i(W_1 W_1^T)\}^{1/2} = 1 + O_p(n^{-1/2})$ and $\epsilon_{ij} = O_p(n^{-1/2})$. Here, $\rho_i$ and $\epsilon_{ij}$ are defined in Theorem 4. Thus, taking limits $d \to \infty$, $n \to \infty$,

$$\frac{\hat{w}_{ij}}{w_{ij}} \to 1. \tag{S3.6}$$

in probability, which in turn implies that $a_j(k) \to 0$ in probability.

All in all, we get

$$R_j(k) \to B_j(k, m), \tag{S3.7}$$

in probability, as $d \to \infty$ and $n \to \infty$. Lemma S3.1 ensures that $B_j(k, m) = \sum_{i=k+1}^m \sigma_i^2 z_{ij}^2 + \tau^2$ is right-skewed. Since $\{(z_{1j}, \ldots, z_{mj}) : j = 1, 2, \ldots\}$ is an i.i.d. sequence of random variables (by Condition 3), $\{B_j(k, m) : j = 1, 2, \ldots\}$ is also i.i.d.

## S3·4. *Proof of Theorem 3*

Note that $\hat{m}(\alpha) = m$ if and only if

$$p_k < \alpha \ \text{ for all } \ k = 0, 1, \ldots, m-1, \ \text{ and } \ p_m > \alpha. \tag{S3.8}$$

The p-value $p_k = p_k(R_1(k), \ldots, R_n(k))$ is computed using the moment-based skewness test (D'Agostino, 1970) and is a continuous function of the sample skewness coefficient $b_1 = m_3/(m_2)^{3/2}$, where $m_r = n^{-1} \sum_{j=1}^n (R_j(k) - \bar{R}_{\cdot}(k))^r$, $\bar{R}_{\cdot}(k) = n^{-1} \sum_{j=1}^n R_j(k)$. In particular,

$$p_k = 1 - \Phi(Z_n), \quad Z_n = \delta_n \log[b_1/\lambda_n + \{b_1^2/\lambda_n^2 + 1\}^{1/2}],$$

and it can be checked that $\lim_{n\to\infty} \delta_n = \infty$ and $\lim_{n\to\infty} \lambda_n = \sqrt{2/3}$. Thus if $b_1 \to b_{\rm lim}$ in probability, then

$$p_k \to \begin{cases} 0, & \text{if } b_{\rm lim} > 0; \\ .5, & \text{if } b_{\rm lim} = 0; \\ 1, & \text{if } b_{\rm lim} < 0, \end{cases} \tag{S3.9}$$

in probability, as $n \to \infty$.

Suppose that $Y_1, \dots, Y_n$ is a random sample from a population whose skewness coefficient $b_{\rm lim}$ is negative (or positive), then $b_1 = b_1(Y_1, \dots, Y_n) \to b_{\rm lim}$, and $p_k(Y_1, \dots, Y_n) \to 0$ (or 1, respectively) in probability as $n \to \infty$. Therefore, the probability of the event (S3.8), for any $\alpha \in (0, 1)$, tends to 1 in the limit $d \to \infty$, $n \to \infty$ if

$$\begin{aligned} &b_1(R_1(k), \dots, R_n(k)) \to b_{(k)} \text{ in probability as } d \to \infty,\ n \to \infty\ (k = 0, \dots, m), \text{ and} \\ &b_{(k)} < 0 \ \text{ for all } \ k = 0, 1, \dots, m-1, \ \text{ and } \ b_{(m)} > 0. \end{aligned} \tag{S3.10}$$

Thus it is enough to show (S3.10). In the following, we use the convention that the notation $O_p(n^{-1/2})$ represent a random variable $Y_n$ if $Y_n = O_p(n^{-1/2})$.

Let $k \in \{0, \dots, m-1\}$. The proof of Theorem 2 leads that for each fixed $n$, $(R_1(k), \dots, R_n(k)) \to (B_1(k, m) + O_p(n^{-1/2}), \dots, B_n(k, m) + O_p(n^{-1/2}))$ in probability as $d \to \infty$. Thus,

$$m_r(R_1(k), \dots, R_n(k)) \to m_r(B_1(k, m), \dots, B_n(k, m)) + O_p(n^{-1/2}), \quad (r = 2, 3)$$

in probability as $d \to \infty$ (by the continuous mapping theorem). Write $m_r^{(B)}(k, m, n) = m_r(B_1(k, m), \dots, B_n(k, m))$. We get

$$b_1(R_1(k), \dots, R_n(k)) \to m_3^{(B)}(k, m, n)/(m_2^{(B)}(k, m, n))^{3/2} + O_p(n^{-1/2}), \tag{S3.11}$$

in probability as $d \to \infty$. Taking the limit $n \to \infty$ on the right hand side of (S3.11), we have

$$b_1(R_1(k), \dots, R_n(k)) \to b_{k,m},$$

in probability, where $b_{k,m} > 0$ is the population skewness coefficient of $B_1(k, m)$ (which is right-skewed, as shown in Theorem 2(iii)). This shows (S3.10) for $k < m$.

Let $k = m$. Then for each fixed $n$,

$$(n(R_1(k) - \tau^2), \dots, n(R_n(k) - \tau^2)) \to (A_1(m) + O_p(n^{-1/2}), \dots, A_n(m) + O_p(n^{-1/2}))$$

in probability as $d \to \infty$. Thus,

$$m_r(R_1(k), \dots, R_n(k)) \to n^{-r} m_r(A_1(m), \dots, A_n(m)) + O_p(n^{-1/2-r}), \quad (r = 2, 3)$$

in probability as $d \to \infty$. Write $m_r^{(A)}(m, n) = m_r(A_1(m), \dots, A_n(m))$. We get

$$b_1(R_1(k), \dots, R_n(k)) \to m_3^{(A)}(m, n)/(m_2^{(A)}(m, n))^{3/2} + O_p(n^{-7/2}), \tag{S3.12}$$

in probability as $d \to \infty$. Taking the limit $n \to \infty$ on the right hand side of (S3.12), we have

$$b_1(R_1(k), \dots, R_n(k)) \to b_m,$$

in probability, where $b_m < 0$ is the population skewness coefficient of $A_1(m)$ (which is left-skewed, as shown in Theorem 2(ii)). This shows (S3.10) for $k = m$.

## S4. NULL DISTRIBUTIONS FOR FIXED $n$

As a supplementary theory, we characterize the null distributions of $R_j(m)$ in the high-dimension, low-sample-size asymptotic scenario, i.e., $d \to \infty$ while $n$ is fixed. Since the sample size $n$ is non-increasing, there exists a non-trivial error caused by the fixed sample size. To characterize the size of this error, we use the following to control errors in the first $m$ estimated principal components. Theorem S4.1 says that, in the limit $d \to \infty$, $R_j(m)$, $m \geq 1$, is a linear combination of a left-skewed random variable $A_{j,n}$ and an error $E_{j,n}$, and that the error $E_{j,n}$ becomes negligible compared to $A_{j,n}$ when $n$ is large.

We say that a nonnegative random variable $X$ is *sub-exponential* with rate factor $a$ if $E(e^{\lambda X}) \leq 1/(1-\lambda/a)$ for all $\lambda \in (0, a)$.

(A) For the pervasive factors $z_{ij}$, $1 \leq i \leq m$, $z_{ij}^2$ is sub-exponential with rate factor $a > 0$.

THEOREM S4.1. *Assume the $m$-factor model under Conditions 1–4 and (A). Let $n > m \geq 0$ be fixed. Then for large $d$,*

*(i) If $m = 0$, then $R_j(0)$ is asymptotically normal.*

*(ii) If $m \geq 1$, then $R_j(m) \to \tau^2 + A_{j,n} + E_{j,n}$ in distribution as $d \to \infty$, where $A_{j,n} = -\frac{\tau^2}{n}\sum_{i=1}^m z_{ij}^2$ is left-skewed, and the error term $E_{j,n}$ is negligible compared to $A_{j,n}$. Precisely, for any fixed $n$ and $\epsilon \in (0,1)$,*

$$pr(|E_{j,n}| < \epsilon |A_{j,n}|) \geq 1 - 2m^2 \exp\left\{-\frac{n}{\sigma_1^2} h\left(\frac{a\sigma_m^4 \epsilon}{8\sigma_1^2 m^2}\right)\right\},$$

*where $h(u) = 1 + u - \sqrt{1+2u}$, for $u > 0$.*

*Proof of Theorem S*4.1. The case (i), where $m = 0$, is obtained by Corollary 1, since $R_j^{(d,0)} = \tilde{R}_j^{(d,0)}$.

For the case (ii), $m \geq 1$, it can be seen from the proof of Corollary 1 that $\tilde{R}_j(m) = \tau^2 + O_p(d^{-1/2})$. By the decomposition $R_j(m) = \tilde{R}_j(m) + a_j(m)$, where $a_j(m) = \frac{1}{d}\sum_{i=1}^m (w_{ij}^2 - \hat{w}_{ij}^2)$, $R_j(m) = \tau^2 + O_p(d^{-1/2}) + a_j(m)$. By Theorem 4(i), conditional to $W_1$, $a_j(m)$ converges in probability to

$$\begin{aligned} w_j^{\mathrm{T}} w_j - w_j^{\mathrm{T}} R S^2 R^{\mathrm{T}} w_j &= w_j^{\mathrm{T}} R \left(I_m - S^2\right) R^{\mathrm{T}} w_j \\ &= -\tau^2 w_j^{\mathrm{T}} R[\mathrm{diag}(1/\lambda_1(W_1W_1^{\mathrm{T}}), \ldots, 1/\lambda_m(W_1W_1^{\mathrm{T}}))]R^{\mathrm{T}} w_j \\ &= -\tau^2 w_j^{\mathrm{T}} (W_1W_1^{\mathrm{T}})^{-1} w_j. \qquad \text{(S4.1)} \end{aligned}$$

Here diag$(a_1, \ldots, a_m)$ denotes the $m \times m$ diagonal matrix with the $i$th diagonal element given by $a_i$ $(i = 1, \ldots, m)$. Denote $\Sigma_{W_1} = \mathrm{diag}(\sigma_1^2, \ldots, \sigma_m^2)$ for the expectation of the $m \times m$ matrix $\frac{1}{n}W_1W_1^{\mathrm{T}}$. Then (S4.1) becomes

$$\begin{aligned} -\tau^2 w_j^{\mathrm{T}} (W_1W_1^{\mathrm{T}})^{-1} w_j &= -\frac{\tau^2}{n} w_j^{\mathrm{T}} (\frac{1}{n}W_1W_1^{\mathrm{T}})^{-1} w_j \\ &= -\frac{\tau^2}{n} w_j^{\mathrm{T}} \left\{\Sigma_{W_1}^{-1} + (\frac{1}{n}W_1W_1^{\mathrm{T}})^{-1} - \Sigma_{W_1}^{-1})\right\} w_j \\ &= A_{j,n} + E_{j,n}, \end{aligned}$$

where $A_{j,n} = -\frac{\tau^2}{n}\sum_{i=1}^m z_{ij}^2$ and $E_{j,n} = -\frac{\tau^2}{n} w_j^{\mathrm{T}} [(\frac{1}{n}W_1W_1^{\mathrm{T}})^{-1} - \Sigma_{W_1}^{-1}] w_j$.

Notice that $A_{j,n}$ is an independent sum of left-skewed random variables. Lemma S3.1 ensures that $A_{j,n}$ is left-skewed.

To give a bound on the error term $E_{j,n}$, we have

$$\begin{aligned}|E_{j,n}| &\leq \frac{\tau^2}{n}\|w_j\|_2^2\|\Sigma_{W_1}^{-1} - (\frac{1}{n}W_1W_1^{\mathrm{T}})^{-1}\|_2 \\ &\leq \frac{\tau^2}{n}(\sum_{i=1}^{m}\sigma_i^2 z_{ij}^2)\|\Sigma_{W_1}^{-1} - (\frac{1}{n}W_1W_1^{\mathrm{T}})^{-1}\|_2 \\ &\leq \sigma_1^2|A_{j,n}|\|\Sigma_{W_1}^{-1} - (\frac{1}{n}W_1W_1^{\mathrm{T}})^{-1}\|_2\end{aligned}$$

So

$$P(|E_{j,n}| > \epsilon|A_{j,n}|) \leq P(\|\Sigma_{W_1}^{-1} - (\frac{1}{n}W_1W_1^{\mathrm{T}})^{-1}\|_2 > \epsilon\sigma_1^{-2}). \tag{S4.2}$$

We will use the following classical result on the error bound of matrix inversion.

THEOREM S4.2. *(Theorem 2.3.4. Golub & Van Loan, 1996) Let $A$ and $E$ be $m \times m$ matrices. If $A$ is nonsingular and $r \equiv \|A^{-1}E\|_p < 1$, then $A + E$ is nonsingular and*

$$\|(A+E)^{-1} - A^{-1}\|_p \leq \frac{\|E\|_p\|A^{-1}\|_p^2}{1-r}.$$

To apply the proceeding theorem with $A = \Sigma_{W_1}$ and $E = \frac{1}{n}W_1W_1^{\mathrm{T}} - \Sigma_{W_1} \equiv \Delta$ for $p = 2$, we need the condition

$$r = \|\Sigma_{W_1}^{-1}\Delta\|_2 \leq \|\Sigma_{W_1}^{-1}\|_2\|\Delta\|_2 = \frac{1}{\sigma_m^2}\|\Delta\|_2 < 1, \tag{S4.3}$$

thus sufficiently,

$$\|\Delta\|_2 < \sigma_m^2. \tag{S4.4}$$

If (S4.4) holds, then using the notation $\nabla \equiv \Sigma_{W_1}^{-1} - (\frac{1}{n}W_1W_1^{\mathrm{T}})^{-1}$, we obtain

$$\|\nabla\|_2 \leq \frac{\sigma_m^{-4}}{1-r}\|\Delta\|_2 \leq \sigma_m^{-4}\|\Delta\|_2. \tag{S4.5}$$

Now, conditioning the probability of (S4.2) by (S4.4), and using the notation $\nabla \equiv \Sigma_{W_1}^{-1} - (\frac{1}{n}W_1W_1^{\mathrm{T}})^{-1}$, and $\epsilon' = \epsilon\sigma_1^{-2}$, we have

$$\begin{aligned}\mathrm{pr}(\|\nabla\|_2 > \epsilon') &= \mathrm{pr}(\|\nabla\|_2 > \epsilon' \mid \|\Delta\|_2 < \sigma_m^2)\mathrm{pr}(\|\Delta\|_2 < \sigma_m^2) \\ &\quad + \mathrm{pr}(\|\nabla\|_2 > \epsilon' \mid \|\Delta\|_2 \geq \sigma_m^2)\mathrm{pr}(\|\Delta\|_2 \geq \sigma_m^2) \\ &\leq \mathrm{pr}(\|\Delta\|_2 > \sigma_m^4\epsilon' \mid \|\Delta\|_2 < \sigma_m^2)\mathrm{pr}(\|\Delta\|_2 < \sigma_m^2) + \mathrm{pr}(\|\Delta\|_2 \geq \sigma_m^2) \quad \text{(S4.6)} \\ &\leq \mathrm{pr}(\sigma_m^4\epsilon' < \|\Delta\|_2 < \sigma_m^2) + \mathrm{pr}(\|\Delta\|_2 \geq \sigma_m^2) \\ &= \mathrm{pr}(\|\Delta\|_2 \geq \sigma_m^4\sigma_1^{-2}\epsilon) \quad \text{(S4.7)}\end{aligned}$$

The last equality is given by the assumptions $\epsilon \in (0, 1)$, $\sigma_1 > \sigma_m$, which in turn leads $\sigma_m^4\epsilon' = \sigma_m^4\sigma_1^{-2}\epsilon < \sigma_m^2$. Theorem S4.2 is used at (S4.6).

Since we know for any square symmetric $\Delta$, $\|\Delta\|_2 \le \|\Delta\|_F = \|\mathrm{vec}(\Delta)\|_2 \le \|\mathrm{vec}(\Delta)\|_1 = \sum_{i=1}^m \sum_{j=1}^m |\Delta_{i,j}|$, we will use element-wise bound for (S4.7). Note that

$$\Delta_{ij} = \begin{cases} n^{-1}\sigma_i^2 \sum_{l=1}^n (z_{il}^2 - 1), & i = j, \\ n^{-1}\sigma_i\sigma_j \sum_{l=1}^n z_{il} z_{jl}, & i \ne j. \end{cases} \tag{S4.8}$$

The assumption (A) ensures that $z_{ij}^2$ $(i = 1, \dots, m)$ is sub-exponential. Note that if $z_{ij}$ is standard normal, then since $E(e^{\lambda z_{ij}^2}) = (1 - 2\lambda)^{-1/2} \le 1/(1 - 2\lambda)$ for $0 < \lambda < 1/2$, $z_{ij}^2$ is sub-exponential. If a random variable $X$ is sub-exponential, then for every positive integer $q$, $E(X^q) \le 2^{q+1}\frac{q!}{a^q}$ (Boucheron et al., 2013).

We will show in Lemma S4.1 that some functions of sub-exponential random variables are *sub-gamma*. For this, we give a definition of sub-gamma random variables. A centered random variable $X - \mu$ with $E(X) = \mu$ is said to be sub-gamma with variance factor $\nu$ and scale factor $c$ if $\log\{E(e^{\lambda X - \lambda\mu})\} \vee \log\{E(e^{-\lambda X + \lambda\mu})\} \le \frac{\lambda^2 \nu}{2(1 - c\lambda)}$ for every $\lambda \in (0, 1/c)$. The collection of such random variables is denoted by $\Gamma(\nu, c)$. It is easily seen that $\Gamma(\nu_1, c_1) \subset \Gamma(\nu_2, c_2)$ for $\nu_1 \le \nu_2$, $c_1 \le c_2$. If $X$ is sub-Gaussian with variance factor $\nu$, then $X \in \Gamma(\nu, 0)$. Finally, if for some positive constants $A$ and $B$,

$$E(X^{2q}) \le q! A^q + (2q)! B^{2q}, \tag{S4.9}$$

for every integer $q \ge 1$, then $X \in \Gamma(4(A + B^2), 2B)$. If $X_i \in \Gamma(\nu, c)$, then $sX_i \in \Gamma(s^2\nu, |s|c)$, and $\sum_{i=1}^n X_i \in \Gamma(n\nu, c)$. Finally, if $X \in \Gamma(\nu, c)$, then for $t > 0$

$$\mathrm{pr}(X > \sqrt{2\nu t} + ct) \vee \mathrm{pr}(-X > \sqrt{2\nu t} + ct) \le e^{-t}, \tag{S4.10}$$

and for $h(u) = 1 + u - \sqrt{1 + 2u}$, for $u > 0$,

$$\mathrm{pr}(X > t) \vee \mathrm{pr}(-X > t) \le e^{-\frac{\nu}{c^2} h(\frac{ct}{\nu})}. \tag{S4.11}$$

LEMMA S4.1. *(i) Suppose a non-negative random variable $X$ with mean $\mu > 0$ is sub-exponential with rate factor a. Then $X - \mu \in \Gamma(\nu, c)$ for $\nu \ge 4^3/a^2$, and $c \ge 8/a$.*

*(ii) Suppose $X$ and $Y$ are independent and sub-exponential with rate factor a. If $E(\sqrt{XY}) = 0$, then $\sqrt{XY} \in \Gamma(\nu, c)$ for $\nu \ge 32/a^2$, and $c \ge 2\sqrt{8}/a$.*

*Proof.* (i) For any integer $q \ge 1$, we have $E(X^q) \le 2^{q+1}\frac{q!}{a^q} \le (4/a)^q q!$. Then

$$E(X - \mu)^{2q} \le E(X^{2q}) \le (4/a)^{2q}(2q)!.$$

Thus, (S4.9) is satisfied with $A = 0$, $B = 4/a$, and we have $X - \mu \in \Gamma(4^3/a^2, 8/a)$.

(ii) Using $(q!)^2 \le 2^{-q}(2q)!$, we have

$$E\{(\sqrt{XY})^{2q}\} = E(X^q)E(Y^q) \le 4^{q+1}\frac{(q!)^2}{a^{2q}} \le 2^{q+2}\frac{(2q)!}{a^{2q}} \le (\sqrt{8}/a)^{2q}(2q)!$$

Thus, (S4.9) is satisfied with $A = 0$, $B = \sqrt{8}/a$, and we have $\sqrt{XY} \in \Gamma(32/a^2, 2\sqrt{8}/a)$. □

To provide upper bounds for (S4.8), we note that by Lemma S4.1, $z_{il}^2 - 1 \in \Gamma(64/a^2, 8/a)$ and $z_{il}z_{jl} \in \Gamma(32/a^2, 2\sqrt{8}/a)$. Therefore, we have for $1 \le i < j \le m$,

$$\Delta_{ii} = n^{-1}\sigma_i^2 \sum_{l=1}^{n}(z_{il}^2 - 1) \in \Gamma\left\{n\left(\frac{\sigma_i^2}{n}\right)^2 \frac{64}{a^2}, \frac{\sigma_i^2}{n}\frac{8}{a}\right\},$$

$$\Delta_{ij} = n^{-1}\sigma_i\sigma_j \sum_{l=1}^{n} z_{il}z_{jl} \in \Gamma\left\{n\left(\frac{\sigma_i\sigma_j}{n}\right)^2 \frac{32}{a^2}, \frac{\sigma_i\sigma_j}{n}\frac{2\sqrt{8}}{a}\right\}.$$

Thus for all $1 \le i, j \le m$,

$$\Delta_{ij} \in \Gamma\left(\frac{64\sigma_1^2}{a^2 n}, \frac{8\sigma_1^2}{an}\right).$$

This gives

$$\text{pr}(|\Delta_{ij}| > t) \le 2\exp\left\{-\frac{n}{\sigma_1^2}h(\frac{at}{8})\right\}, \tag{S4.12}$$

$$\text{pr}(|\Delta_{ij}| > \frac{8\sqrt{2}\sigma_1}{a\sqrt{n}}\sqrt{t} + \frac{8\sigma_1^2}{an}t) \le 2e^{-t}. \tag{S4.13}$$

Combining (S4.7) and (S4.12),

$$\begin{aligned}
\text{pr}(\|\nabla\|_2 > \epsilon\sigma_1^{-2}) &\le \text{pr}(\|\Delta\|_2 > \sigma_m^4\sigma_1^{-2}\epsilon) \\
&\le \sum_{i,j}\text{pr}(|\Delta_{ij}| > \frac{\sigma_m^4\epsilon}{\sigma_1^2 m^2}) \\
&\le 2m^2\exp\left\{-\frac{n}{\sigma_1^2}h\left(\frac{a\sigma_m^4\epsilon}{8\sigma_1^2 m^2}\right)\right\}.
\end{aligned}$$

This concludes Section S4. Supplementary material continues on next page.

## S5. EMPIRICAL DISTRIBUTIONS OF P-VALUE SEQUENCES

The empirical sampling distributions of the p-values $p_k^R$ and $p_k^D$ in Fig. S1 help us to understand the distributions of $R_j(k)$ for finite $d$ and $n$.

Figure S1 confirms the theoretical null distributions in Theorem 2, in the finite dimension. The p-values in the figure are computed from random samples of the model described in main article Section 4.3 with $(d, n, s, g, \beta) = (2500, 100, 0.2, 1, 0)$. For $m = 0$, $p_0^R$ and $p_0^D$ exhibit the uniform null distribution as expected (shown in the first boxplot in each of top panels). For $m = 3$, $R_j(3)$ is left-skewed, confirmed by the large values of $p_3^R$ and $p_3^D$ shown in the fourth $(k = 3)$ boxplot in each of bottom panels. When testing $H_k$ for $k$ larger than the true $m$, the finite-dimensional empirical distribution of $R_j(k)$ is left-skewed, as shown in the $(m+1)$th to tenth boxplots in each panel.

The empirical alternative distributions of the p-values under $H_{a,k} : m \geq k$, $k = 0, 1, 2$, can be found in the first three boxplots in each of bottom panels. In particular, we observe that $R_j(k)$, for $k$ smaller than the true number of components, is right-skewed with high probability.

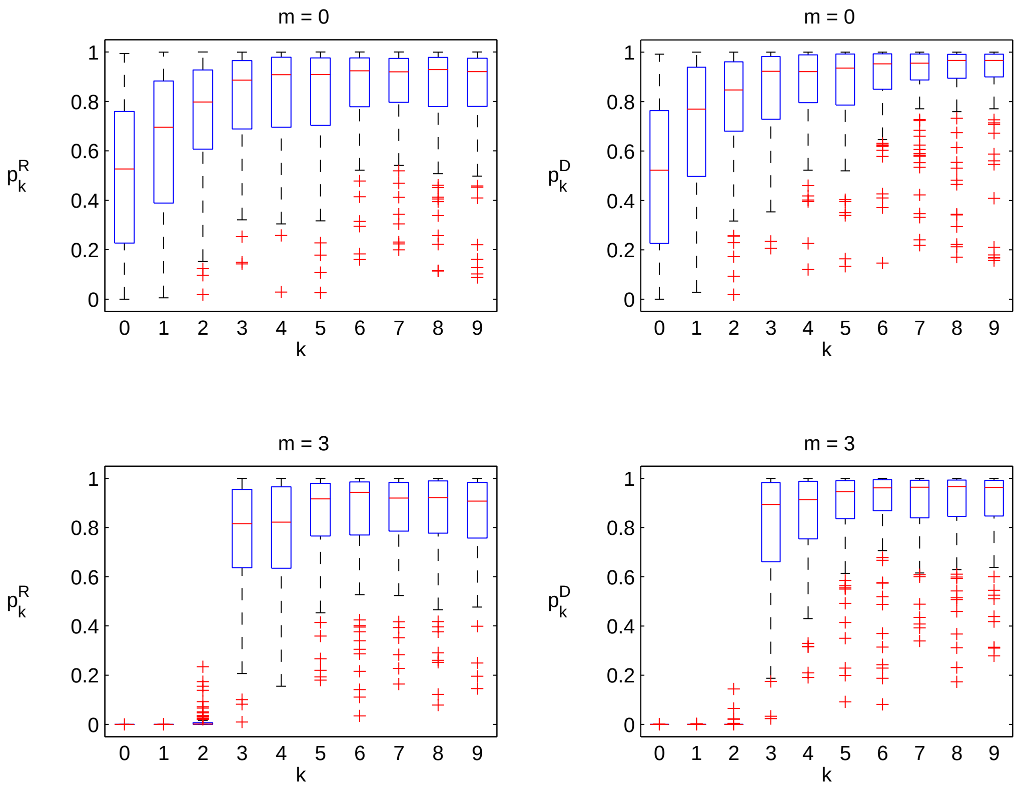


Fig. S1. Finite-dimensional sampling distributions of $p_k^R$ and $p_k^D$. For the global null ($m = 0$, top panels), all p-values at $k = 0$ appear to have the uniform distribution. For $m = 3$ in the bottom panels, the sequences of $p_k^R$ and $p_k^D$ show a sharp transition from small values (representing right-skewness) to large values (representing left-skewness) at $k = 3$.

# S6. A MODIFIED ESTIMATOR FOR THE NUMBER OF COMPONENTS, BASED ON BAI & NG (2002)

As referenced in Section 5.1, we describe a modified estimator based on an information criterion suggested in Bai & Ng (2002). We use this modified estimator in our empirical studies.

Bai & Ng (2002) proposed several information criteria. For example, a criterion denoted by $\text{IC}_{p_1}(k)$, for the candidate number of component $k$, is defined by

$$\text{IC}_{p_1}(k) = \log\left(\frac{1}{n}\sum_{j=1}^{n} R_j(k)\right) + k\left(\frac{d+n}{dn}\right)\log\left(\frac{dn}{d+n}\right), \tag{S6.1}$$

where

$$R_j(k) = \frac{1}{d}\left\| X_j - \sum_{i=1}^{k} \hat{u}_i\hat{u}_i^{\mathrm{T}} X_j \right\|_2^2, \quad 1 \le j \le n. \tag{S6.2}$$

Bai and Ng argued in their Theorem 2 and Corollary 1 of Bai & Ng (2002) that the estimator $\hat{m}_{\text{IC}_{p_1}} = \text{argmin}_{0\le k\le k_{\text{max}}}\text{IC}_{p_1}(k)$ is a consistent estimator of $m$ if $k_{\text{max}} > m$ and under some regularity conditions. Bai & Ng (2002) recommended to use $k_{\text{max}} = \min(d, n)$.

However, we found using both the recommended $k_{\text{max}} = \min(d, n)$ and a slightly-modified $k_{\text{max}} = \min(d, n-1)$ unsatisfactory for most of the real data analysis and simulation studies. In particular, setting $k_{\text{max}} = n - 1 = \min(d, n-1)$ always provides estimates $\hat{m} = n - 1$, not only when using $\text{IC}_{p_1}$ but also using any of the proposed information criterion. To elaborate this, we applied the methods of Bai & Ng (2002) to the Leukemia data (Golub et al., 1999), and obtained the graphs of information criterion. Figure S2 contains these graphs, showing that minima are achieved at $k = n - 1$ for all criteria. For this and many other data examples we tested, the information measures $\text{PC}_{p1}$, $\text{PC}_{p1}$, $\text{PC}_{p1}$, AIC and BIC are always decreasing (these measures are defined in Bai & Ng (2002)). Fortunately, the information criterion $\text{IC}_{p_1}$ typically exhibits a local minimum, as shown in Fig. S2, which provides a reasonable estimate for $m$.

To summarize, we use the local minimum, closest to the zero, of $\text{IC}_{p_1}$.

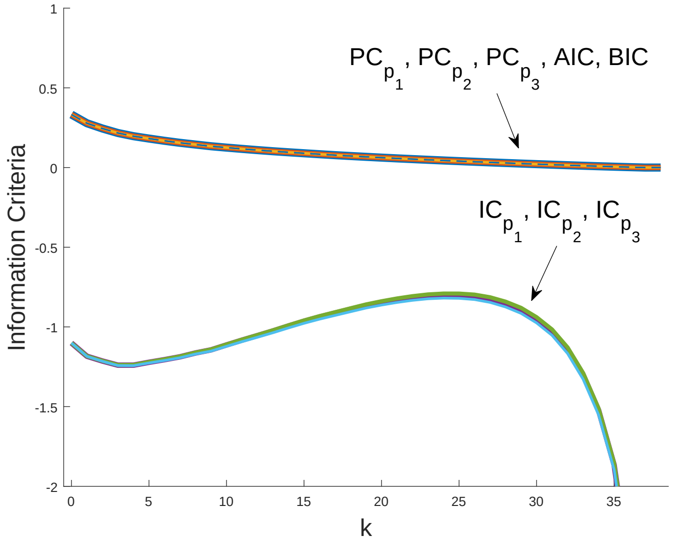


Fig. S2. The methods of Bai & Ng (2002) give the estimate $\hat{m} = n - 1$, when $k_{\text{max}}$ is set as recommended.

## S7. EXTENDED SIMULATION RESULTS

As referenced in Section 5.3, we supply more simulation results. We set for each dimension $d$, and for $s > 0$, representing a signal strength, $0 \leq \beta < 1/2$, representing a decay rate of variances in noise components, the eigenvalues of $\Sigma_d$ are modeled as

$$\lambda_i = \begin{cases} \sigma_i^2 d, \quad \sigma_i^2 = s^2\{1 + g(m-i)\}, \, i = 1, \ldots, m; \\ \tau_\beta i^{-\beta}, \qquad\qquad\qquad\qquad\qquad m < i \leq d, \end{cases} \tag{S7.1}$$

where $\tau_\beta = (\sum_{i=m+1}^{d} i^{-\beta}/(d-m))^{-1}$ is used to ensure that the average of $\lambda_i$, $i > m$, is 1. The performances of the proposed estimators $\hat{m}_R$ and $\hat{m}_D$ are compared with competing methods: $\hat{m}_L$, the estimator of Leek (2011); $\hat{m}_{KN}$, the estimator of Kritchman & Nadler (2008); $\hat{m}_{PY}$, the estimator of Passemier & Yao (2014); $\hat{m}_{BN}$, the estimator defined in supplementary Section 6, based on Bai & Ng (2002).

Our additional simulation results are generated from six cases (Cases A–F), as described below. We use $\alpha = 0.1$ for $\hat{m}_R$ and $\hat{m}_D$. In addition, we provide supplement graphics of the four simulation settings in the main article Section 4.3, with varying $\alpha$ (Case G). In particular, Fig. S7 provides a visual evidence that $\hat{m}_R$ and $\hat{m}_D$ are stable for arbitrary choices of $\alpha$.

Case A (Ideal case, increasing dimensions) These models have the equal tail eigenvalues, $\lambda_i \equiv 1$ for all $i > m$. Our estimators $\hat{m}_R$ and $\hat{m}_D$ show better performance for higher dimensionality, as expected from the theoretical results. The estimators of Leek (2011) and Bai & Ng (2002) are underestimating, while Kritchman & Nadler (2008) and Passemier & Yao (2014) show the smallest mean squared errors in general. The performances of the estimators are graphically summarized in Fig. S3.

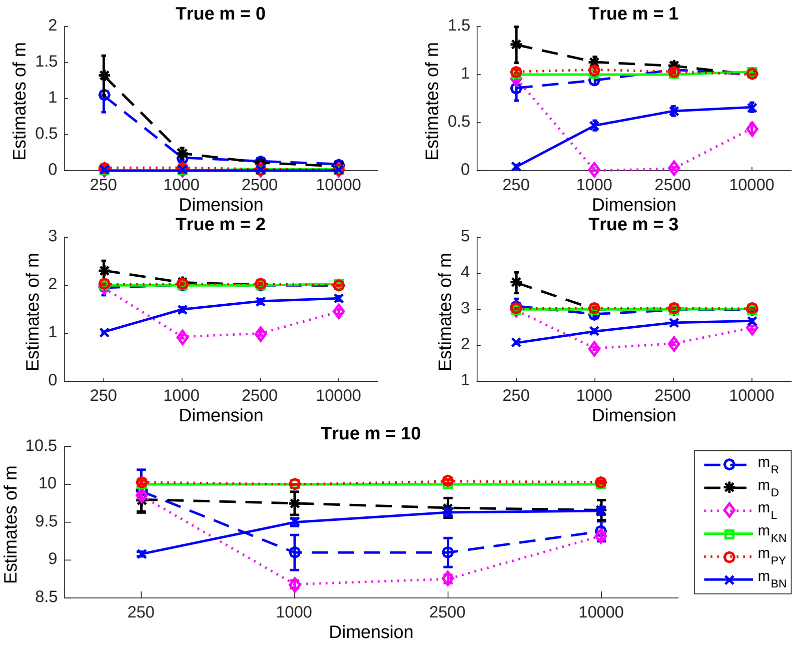


Fig. S3. The performances of estimators in the ideal case for increasing dimensions. $m = 0, 1, 2, 3, 10$, $(s, g, \beta) = (0.2, 1, 0)$, for $d = 250, 1000, 2500, 10000$ and $n = 100$. We use the standard normal distribution for sampling of standardized scores.

Case B (Unequal eigenvalues, increasing dimensions) In the settings with non-zero $\beta$, the methods of Kritchman & Nadler (2008) and Passemier & Yao (2014) tend to overestimate. In particular for the method of Kritchman & Nadler (2008), the bias increases as $d \to \infty$. This is because, for any $\beta > 0$, the critical equal-eigenvalue assumption for $\hat{m}_{KN}$ for consistency is not satisfied. On the other hand, the methods of Bai & Ng (2002) and Leek (2011) often lead to underestimation of $m$, even for large $d$. The results from these models are graphically summarized in Fig. S4.

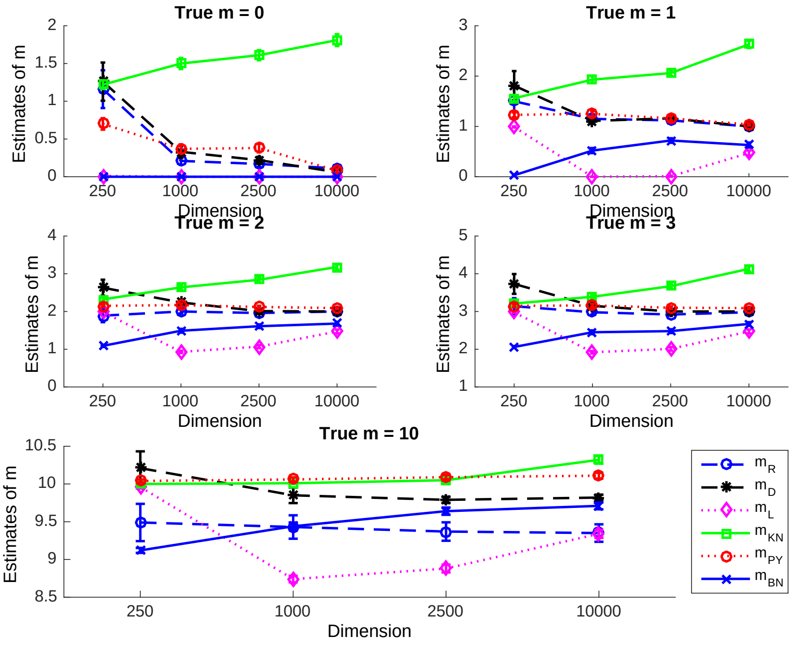


Fig. S4. The performances of estimators in polynomially-decreasing tail-eigenvalue models. $m = 0, 1, 2, 3, 10$, $(s, g, \beta) = (0.2, 1, 0.3)$, for $d = 250, 1000, 2500, 10000$ and $n = 100$. We use the standard normal distribution for sampling of standardized scores.

Case C (Increasing signal strength and separation) All methods considered perform better for larger signal strength of the leading eigenvalues. For large enough gap between leading eigenvalues, all methods are robust to different size of the gap $g$. If $g = 0$, the leading eigenvalues are all equal. For an equal eigenvalue model, both the methods of Kritchman & Nadler (2008) and Passemier & Yao (2014) perform better than other methods. See Fig. S5.

Case D (Large number of $m$) As the dimension and the sample size increase, our estimator $\hat{m}_D$ performs the best and appears to converge to the true value at $m = 30$ or 50, as shown in Table S1. On the other hand, our estimator $\hat{m}_R$ generally underestimates. The estimaors of Kritchman & Nadler and Passemier & Yao overestimate, while those of Bai & Ng and Leek underestimate. This observation is also reported in the main article, and is consistent with the findings from Fig. 2 of the main article and Fig. S7.

Case E (Smaller signal-to-noise ratios) To witness the performances of estimators in "challenging" situations, we keep the principal component variances in the first $m$ components small. In Subcases (a) and (c) used in Fig. S6 and Tab. S2, we set $\lambda_i = 2$ $(i = 1, \ldots, m)$ and $\lambda_i = 1$ $(i > m)$. In Subcases (b), (d) and (e), we use (S7.1) with $(s, g, \beta) = (0.05, 0.05, 0.5)$, which is more challenging to estimate $m$ than Subcases (a) and (c) for all of the estimators consid-

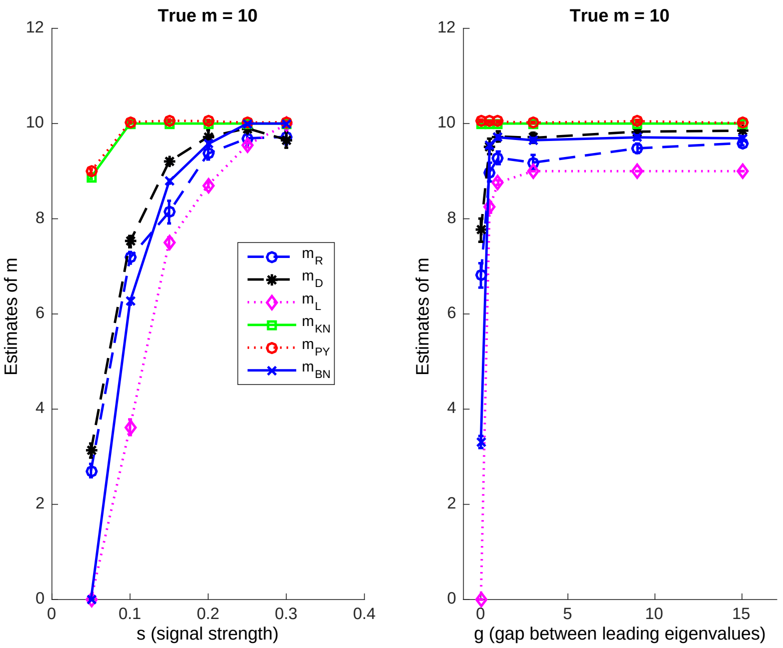


Fig. S5. (left) Increasing signal strength $s = 0.05, 0.1, 0.15, 0.2, 0.25, 0.3$ for fixed $m = 10$, $g = 1$, $\beta = 0$, $d = 2500$ and $n = 100$. (right) Various values of gap between leading eigenvalues $g = 0, 1, 2, 3, 9, 15$ for fixed $m = 10$, $s = 0.2$, $\beta = 0$, $d = 2500$ and $n = 100$.

Table S1. *The performances of estimators in models with large number of true components. Data are generated from Setting 4, in the main article Section 4.3, but with $m = 30, 50$.*

| m | d | n | $\hat{m}_D$ | $\hat{m}_R$ | $\hat{m}_{KN}$ | $\hat{m}_{PY}$ | $\hat{m}_L$ | $\hat{m}_{BN}$ |
|---|---|---|---|---|---|---|---|---|
| 30 | 10000 | 100 | 16.3(4.5) | 15.43(3.48) | 36.7(1.7) | **33.2(1.7)** | 15.0(2.1) | 19.0(1.8) |
| | 20000 | 250 | **29.3(2.4)** | 25.38(2.69) | 47.1(2.7) | 35.8(2.7) | 22.4(3.4) | 27.0(0.8) |
| 50 | 10000 | 100 | 19.7(6.7) | 18.07(5.04) | 53.1(1.2) | **52.7(1.3)** | 28.7(2.7) | 38.9(1.7) |
| | 20000 | 250 | **47.9(3.5)** | 38.89(6.73) | 63.4(2.6) | 56.2(2.2) | 41.3(4.1) | 47.2(0.7) |

$\hat{m}_R$ our estimator using the triples test; $\hat{m}_D$ our estimator using the skewness test; $\hat{m}_L$, Leek (2011) method; $\hat{m}_{KN}$, Kritchman & Nadler (2008) method; $\hat{m}_{PY}$, Passemier & Yao (2014) method; $\hat{m}_{BN}$, Bai & Ng (2002) method.

ered. Figure S6 compares the population variances and empirical variances, to give a visual impression of the difficulty of the task. Our estimators $\hat{m}_D$ and $\hat{m}_R$ underestimate $m$, while Kritchman & Nadler and Passemier & Yao estimators provide better estimates. We emphasize that even though Kritchman & Nadler and Passemier & Yao estimates are generally closer to the true number of components than others (e.g., in Subcase (c), Tab. S2, $\hat{m}_{KN} \approx 13$ is closest to $m = 30$), it is almost impossible to obtain any reasonable estimate of $u_i$, the $i$th principal component directions, for any $i$ large (for example, $\hat{u}_{10}^{\mathrm{T}} u_{10} \approx 0$). On the other hand, our estimators $\hat{m}_D$ and $\hat{m}_R$ reflect the fact that $\hat{u}_i$ is typically orthogonal to $u_i$ (thus reasonable to discard) for almost all $i$.

Case F (Conventional $n > d$ cases) Our proposal is specifically designed for the $d > n$ case, and does not aim to handle the conventional large-sample-size, low-dimension situation ($n > d$) or the moderate-sample-size, moderate-dimension situation ($n \approx d$). Nevertheless, our estimators

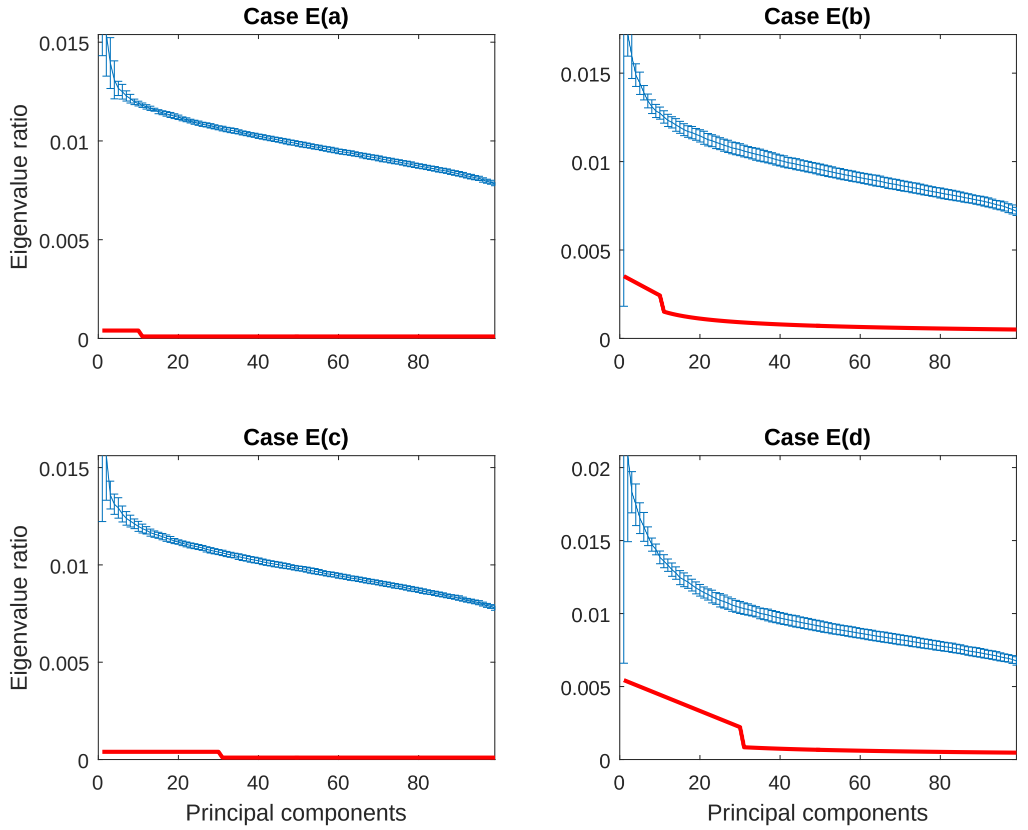


Fig. S6. Models used in Case E and Table S2. True principal component variance ratios (ratio of the $i$th component variance and the total variance) are shown as the red curves. Eigenvalue ratios from the empirical covariances are shown as blue curves (mean $\pm$ standard deviation from 100 repetitions). Case (e) is omitted, as it is similar to Case (d).

Table S2. *The performances of estimators in models with smaller signal-to-noise ratio. We use the $t_3$ distribution for sampling of standardized scores.*

| Case | m | d | n | $\hat{m}_D$ | $\hat{m}_R$ | $\hat{m}_{KN}$ | $\hat{m}_{PY}$ | $\hat{m}_L$ | $\hat{m}_{BN}$ |
|---|---|---|---|---|---|---|---|---|---|
| E(a) | 10 | 10000 | 100 | 1.1(0.3) | 3.00(0.8) | **12.9(2.2)** | 4.1(1.8) | 0.0(0.2) | 0.0(0.2) |
| E(b) | 10 | 10000 | 100 | 1.5(0.6) | 3.52(0.8) | 26.0(1.6) | **6.7(2.9)** | 0.1(0.3) | 0.1(0.3) |
| E(c) | 30 | 10000 | 100 | 1.1(0.3) | 2.89(0.8) | **12.9(1.7)** | 3.9(2.1) | 0.0(0.2) | 0.1(0.3) |
| E(d) | 30 | 10000 | 100 | 2.1(1.1) | 4.14(1.4) | **32.5(1.6)** | 11.5(3.7) | 0.1(0.3) | 0.1(0.3) |
| | | 20000 | 250 | 8.7(4.3) | 11.0(3.2) | 60.9(2.0) | **32.8(5.9)** | 0.0(0.2) | 0.1(0.4) |
| E(e) | 50 | 10000 | 100 | 3.2(1.5) | 5.3(1.5) | **40.6(1.2)** | 16.9(4.7) | 0.2(0.4) | 0.2(0.4) |
| | | 20000 | 250 | 13.2(6.6) | 12.2(4.4) | 71.3(2.3) | **48.0(8.1)** | 0.1(0.4) | 0.3(0.5) |

are still defined, and we empirically observe how the estimators behave in the $n > d$ case. Our simulation setting and results can be found in Tab. S3. There, our estimators $\hat{m}_D$ and $\hat{m}_R$ generally grow as $n$ increases (even beyond $m$). To interpret this, we first recall that $\hat{m}_D < k$ (or $\hat{m}_R < k$) if, heuristically, the $k$th estimated component appears to be noise. Generally, the larger the sample size, the better the component estimates become. Thus, it may be possible that the overestimation is caused by the increasing number of "useful" principal components as $n$ increasing. On the other hand, the asymptotic normality needed in the application of the skewness test (that leads to $\hat{m}_D$) is not satisfied in these moderately-large $d$ situations.

(The asymptotic normality is satisfied for large $d$.) Thus, with large sample sizes, we can expect that the p-values used in the computation of $\hat{m}_D$ tend to be small, leading to the overestimation by $\hat{m}_D$. This can partially explain the observation that $\hat{m}_D$ tends to be larger than $\hat{m}_R$, which is computed from the nonparametric triples test, in most cases with large sample sizes. Moreover, in the $n > d$ case, the asymptotic skewness of residuals does not hold (since the degree of overestimation of $\lambda_i$ is lessened), which is central in our method. In the all cases considered here, Kritchman & Nadler and Passemier & Yao estimators perform best. Leek's estimator is also designed to work well only for the high-dimension, low-sample-size situation, and has a tendency to underestimate.

Table S3. *The performances of estimators for moderate dimension and increasing sample size.*

| Case | m | d | n | $\hat{m}_D$ | $\hat{m}_R$ | $\hat{m}_{KN}$ | $\hat{m}_{PY}$ | $\hat{m}_L$ | $\hat{m}_{BN}$ |
|---|---|---|---|---|---|---|---|---|---|
| Case F(a) | 10 | 100 | 250 | 27.6(26.7) | 9.2( 2.8) | **10.0(0.1)** | **10.0(0.1)** | 7.6 (0.7) | 9(0) |
| | | | 500 | 69.9(30.2) | 9.1( 1.8) | **10.0(0.1)** | **10.0(0.1)** | 0(0) | 9.0(0.1) |
| | | | 1000 | 84.8(19.1) | 9.2( 2.1) | **10.1(0.2)** | 10.0(0.3) | 0(0) | 9.0(0.1) |
| | 30 | 100 | 250 | 46.8(22.4) | 9.5(11.2) | **30(0)** | **30.0(0.1)** | 26.9(1.1) | 29.4(0.5) |
| | | | 500 | 82.9(18.0) | 9.0(10.9) | **30(0)** | **30.0(0.1)** | 15.4(3.8) | 29.8(0.3) |
| | | | 1000 | 99 (0) | 7.4( 9.9) | **30.0(0.1)** | **30.0(0.1)** | 0(0) | **30(0)** |
| Case F(b) | 10 | 100 | 250 | 67.1(23.2) | 31.8(9.0) | **11.1(1.5)** | 6.4(2.1) | 0.2(0.4) | 0.7(0.8) |
| | | | 500 | 99(0) | 57.8(17.1) | 14.4(1.7) | **8.8(2.3)** | 0.0(0.1) | 0.9(1.0) |
| | | | 1000 | 99(0) | 81.7(17.1) | 18.5(2.3) | **9.8(2.0)** | 0(0) | 0.8(0.9) |
| | 30 | 100 | 250 | 81.2(14.1) | 47.4( 9.9) | **28.6(1.4)** | 22.5(4.9) | 5.1(2.9) | 9.6(6.3) |
| | | | 500 | 99(0) | 71.8(13.7) | **31.4(1.5)** | 27.9(2.7) | 0.1(0.3) | 19.4(4.0) |
| | | | 1000 | 99(0) | 87.6(7.00) | 33.6(1.8) | **29.3(3.1)** | 0(0) | 21.3(4.6) |
| Case F(c) | 10 | 1000 | 100 | 2.4(0.9) | 4.2(1.1) | **7.3(1.6)** | 2.9(1.7) | 0.2(0.4) | 0.2(0.4) |
| | | | 250 | 6.3(2.0) | 8.5(3.0) | **10.5(1.9)** | 4.1(2.2) | 0.1(0.4) | 0.3(0.5) |
| | | | 500 | 19.6(5.1) | 17.9(7.0) | **14.8(2.4)** | 4.9(2.1) | 0.7(0.9) | 0.4(0.7) |
| | | | 2000 | 169.9(26.7) | 77.6(28.9) | 26.0(2.6) | **10.7(3.9)** | 0.0(0.2) | 0.3(0.6) |
| | 30 | 1000 | 100 | 2.8(1.2) | 4.5(1.5) | **10.5(1.7)** | 3.4(1.6) | 0.1(0.3) | 0.2(0.4) |
| | | | 250 | 10.4(3.3) | 11.6(4.6) | **18.2(1.8)** | 5.6(2.2) | 0.2(0.4) | 0.3(0.5) |
| | | | 500 | **30.4(5.3)** | 27.0(10.1) | 27.6(2.2) | 7.2(2.9) | 0.8(0.8) | 0.4(0.6) |
| | | | 2000 | 189.4(28.1) | 92.7(31.4) | 43.2(2.5) | **21.4(8.0)** | 0.1(0.3) | 0.4(0.6) |

Case F(a): $(s, g, \beta) = (0.2, 1.0.3)$, normally distributed scores, as defines as Case I in the main article Section 4.3; Case F(b): $(s, g, \beta) = (0.2, 1.0.3)$, scores from $t_3$ distribution, as defined as Case IV in the main article Section 4.3; Case F(c): $(s, g, \beta) = (0.05, 0.05, 0.5)$, scores from $t_3$ distribution, as defined as Case E(b) above; See Table S1 for symbols.

Case G Supplement graphics of the four simulation settings in the main article Section 4.3. We report the variation of our estimates $\hat{m}_R$ and $\hat{m}_D$, depending on various values of $\alpha$. As shown in Figs. S7, for any choice of $\alpha \in [0.1, 0.5]$, the proposed estimator shows the best overall performance.

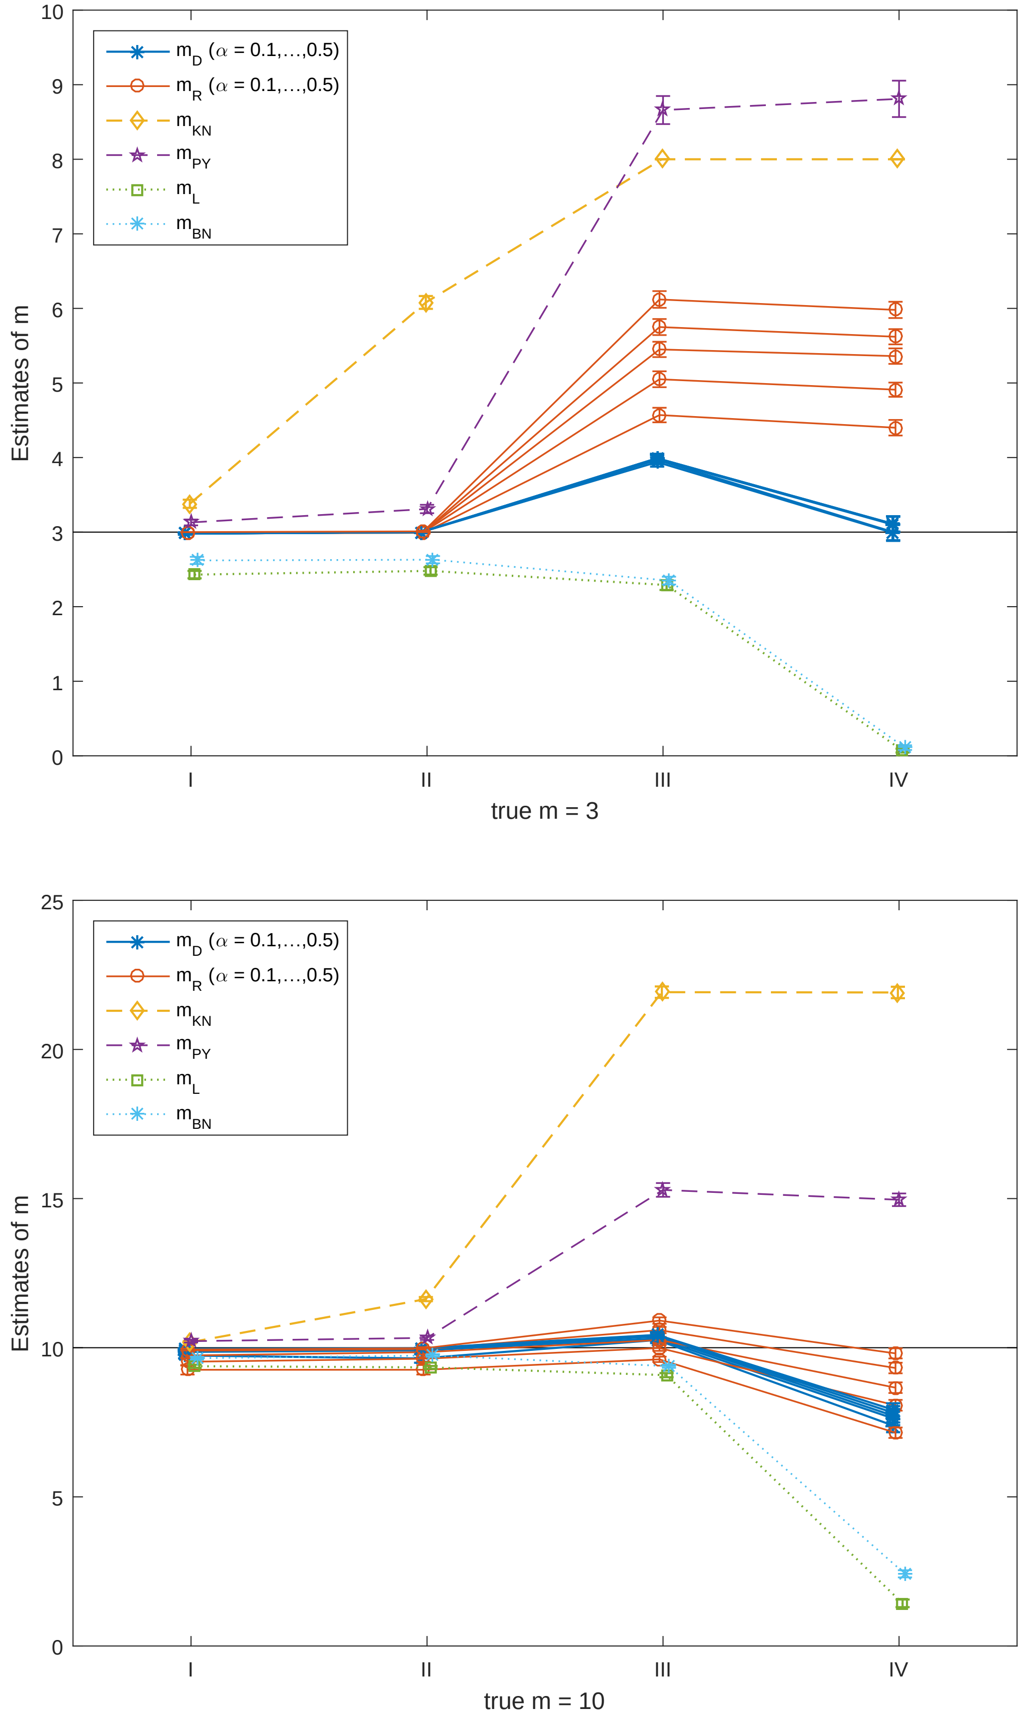


Fig. S7. Robustness of $\hat{m}_R$ and $\hat{m}_D$ against arbitrary choice of $\alpha$. This figure is an extension of main article Figure 2.

## S8. REAL DATA EXAMPLES WITH AUGMENTED NOISES

We further demonstrate the performance of our estimators and the usefulness of PC scores discussed in main article Section 5, using the leukemia data of Golub et al. (1999). There are $p = 3051$ variables of $n = 38$ patients, 27 with acute lymphocytic leukemia (ALL), 11 with acute myeloid leukemia (AML). An application of principal component analysis clearly shows that the first few component scores are important in making distinction between ALL and AML, as shown in Fig. S8. We designed a simulation study to visualize the usefulness of the principal scores, and to demonstrate the robustness of $\hat{m}_D$ against added noise variables. For this, the original data matrix, say $\mathcal{X}$, is augmented by a large number of noise variables. In particular, we generated for $c = 1000$,

$$\mathcal{X}_\ell = \left(\mathcal{X},\, Z_{c\ell} + \mathcal{X}^*_{c\ell}\right),\ \ell = 0, 1, 2, 3, 4,$$

where the first $p$ columns of $\mathcal{X}_\ell$ are those of $\mathcal{X}$, but the latter $c\ell$ rows are the sum of independent noises $Z_{c\ell}$ following $N(0, 1)$ and randomly chosen columns $\mathcal{X}^*_{c\ell}$ from $\mathcal{X}$, with replacement. For each $\ell$, we estimated the number of components by the six methods listed in main article Section 4.1, and collected the corresponding sample principal component scores. As shown in Fig. S8, while the dimension increases, $\hat{m}_D$ (together with $\hat{m}_{KN}$ and $\hat{m}_{PY}$) provides stable estimates for the number of components, that is, it does not degenerate to 0 or 1. Throughout all dimensions, $\hat{m}_R$ remains to be 1, and is excluded from the figure.

To examine whether the estimates $\hat{m}_D$ are reasonable, the first four components in $\mathcal{X}_\ell$ are visualized in the bottom panels of Fig. S8. For simplicity, we chose $\ell = 0, 4$. Based on the findings in main article Section 5, we believe that the effective number $m$ of components must be greater than 4. Since the first four principal scores from $\mathcal{X}_0$ and $\mathcal{X}_4$ show similar patterns, they are from effective components; the scores from $\mathcal{X}_4$ are as useful as those of $\mathcal{X}_0$. In this sense, the estimator $\hat{m}_D$ may be viewed as more "robust" against added noises for this data set than other estimators such as $\hat{m}_L$ and $\hat{m}_{BN}$. On the other hand, we believe the true number $m$ does not exceed 10, because the higher-order scores from $\mathcal{X}_4$ do not exhibit the same pattern as those from $\mathcal{X}_0$, which implies that they are mostly accumulated noises. The scatter plots of higher-order scores are reported in the next section.

In Fig. S9 we further visualize the changes of projection scores of the first to 16th principal components, for the experiment above. In Fig. S9, it is shown that the first few principal component scores are robust to added noises, and exhibit similar patterns when noises are added. On the other hand, the original patterns of higher-order principal component scores are simply lost when noises are excessively added. This is shown, for example, through the 11th and 12th principal component scores. Our method provides a reasonable number of components, $\hat{m}_D = 5$, for the noise-augmented data $\mathcal{X}_4$. In comparison, $\hat{m}_L = 1$ and $\hat{m}_{BN} = 0$ are clearly underestimating, while $\hat{m}_{KN}$ and $\hat{m}_{PY}$ are overestimating the effective number of components.

Finally, we report the sequences of empirical p-values $p_k^R$ and $p_k^D$ for the original leukemia data. As seen in Table 1, there is a discrepancy between $\hat{m}_R = 1$ and $\hat{m}_D = 9$ for the leukemia data. This difference can be explained by the p-value sequences depicted in Fig. S10. The p-value $p_1^R$ is slightly large than the critical value $\alpha = 0.1$. However, for each $k = 2, 3, 4$ and 5, $p_k^R$ is in fact smaller than 0.1, suggesting that the true $m > 5$. Visual inspection of $p_k^R$ in Fig. S10 suggests $\hat{m} = 6$ or 9. For noise-augmented data sets, we also observed this phenomenon ($p_1^R > \alpha$, $p_k^R < \alpha$ for $1 \neq k \leq 5$). Thus, the estimates $\hat{m}_R$ are 1 for all data sets.

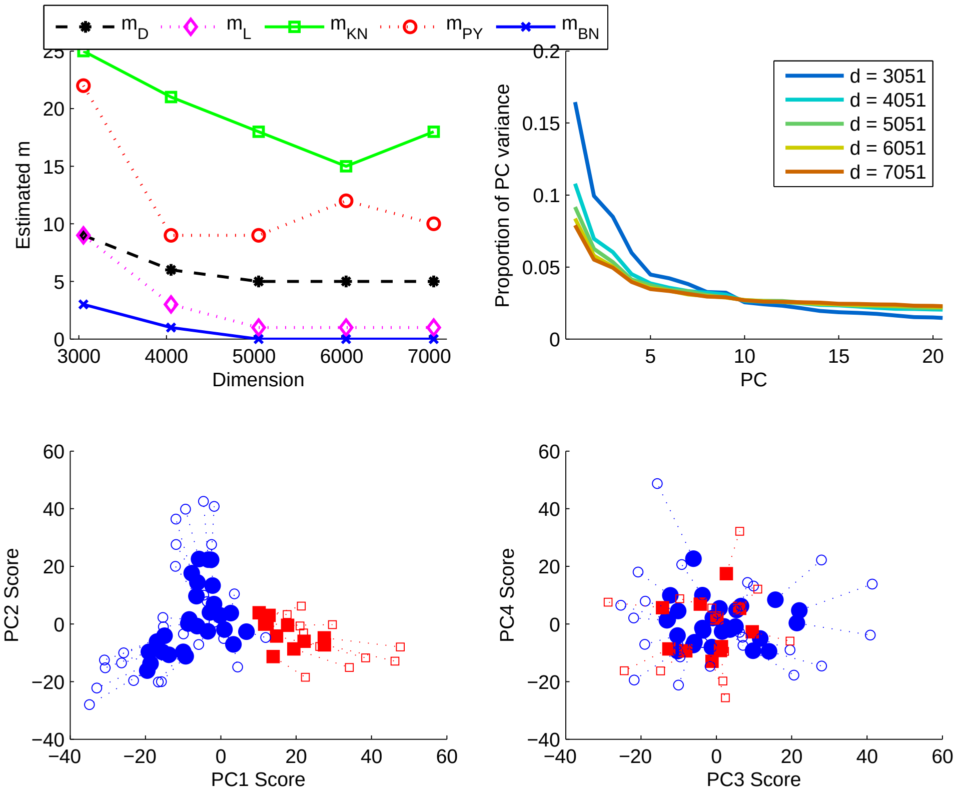


Fig. S8. Noise-augmented leukemia data. (Top left) Estimated number of components, $m$, from $\mathcal{X}_\ell$ against the dimensions of $\mathcal{X}_\ell$. (Top right) Sample scree plots from eigenanalysis. (Bottom panels) Scores plot for PC1-2 and PC3-4. Filled symbols are scores from $\mathcal{X}_0$ and void symbols are scores from $\mathcal{X}_4$. Two points corresponding to the same subject are joined by a dotted line. Different colors represent different subtypes of leukemia.

## References


Bai, J. & Ng, S. (2002). Determining the number of factors in approximate factor models. *Econometrica* **70**, 191–221.

Boucheron, S., Lugosi, G. & Massart, P. (2013). *Concentration inequalities: A nonasymptotic theory of independence*. OUP Oxford.

D'Agostino, R. B. (1970). Transformation to normality of the null distribution of g1. *Biometrika* , 679–681.

Demmel, J. (1992). The componentwise distance to the nearest singular matrix. *SIAM J. Matrix Anal. Appl.* **13**, 10–19.

Golub, G. H. & Van Loan, C. F. (1996). *Matrix computations*. Johns Hopkins Studies in the Mathematical Sciences. Baltimore, MD: Johns Hopkins University Press, 3rd ed.

Golub, T. R., Slonim, D. K., Tamayo, P., Huard, C., Gaasenbeek, M., Mesirov, J. P., Coller, H., Loh, M. L., Downing, J. R., Caligiuri, M. a., Bloomfield, C. D. & Lander, E. S. (1999). Molecular classification of cancer: class discovery and class prediction by gene expression monitoring. *Science* **286**, 531–537.

Hellton, K. H. & Thoresen, M. (2017). When and why are principal component scores a good tool for visualizing high-dimensional data? *Scand. J. Stat* , to appear.

Jung, S., Sen, A. & Marron, J. (2012). Boundary behavior in High Dimension, Low Sample Size asymptotics of PCA. *J. Multivar. Anal.* **109**, 190–203.

Kritchman, S. & Nadler, B. (2008). Determining the number of components in a factor model from limited noisy data. *Chemometr. Intell. Lab.* **94**, 19–32.

Leek, J. T. (2011). Asymptotic conditional singular value decomposition for high-dimensional genomic data. *Biometrics* **67**, 344–352.

Muirhead, R. J. (1982). *Aspects of multivariate statistical theory*. New York: John Wiley & Sons Inc. Wiley Series in Probability and Mathematical Statistics.

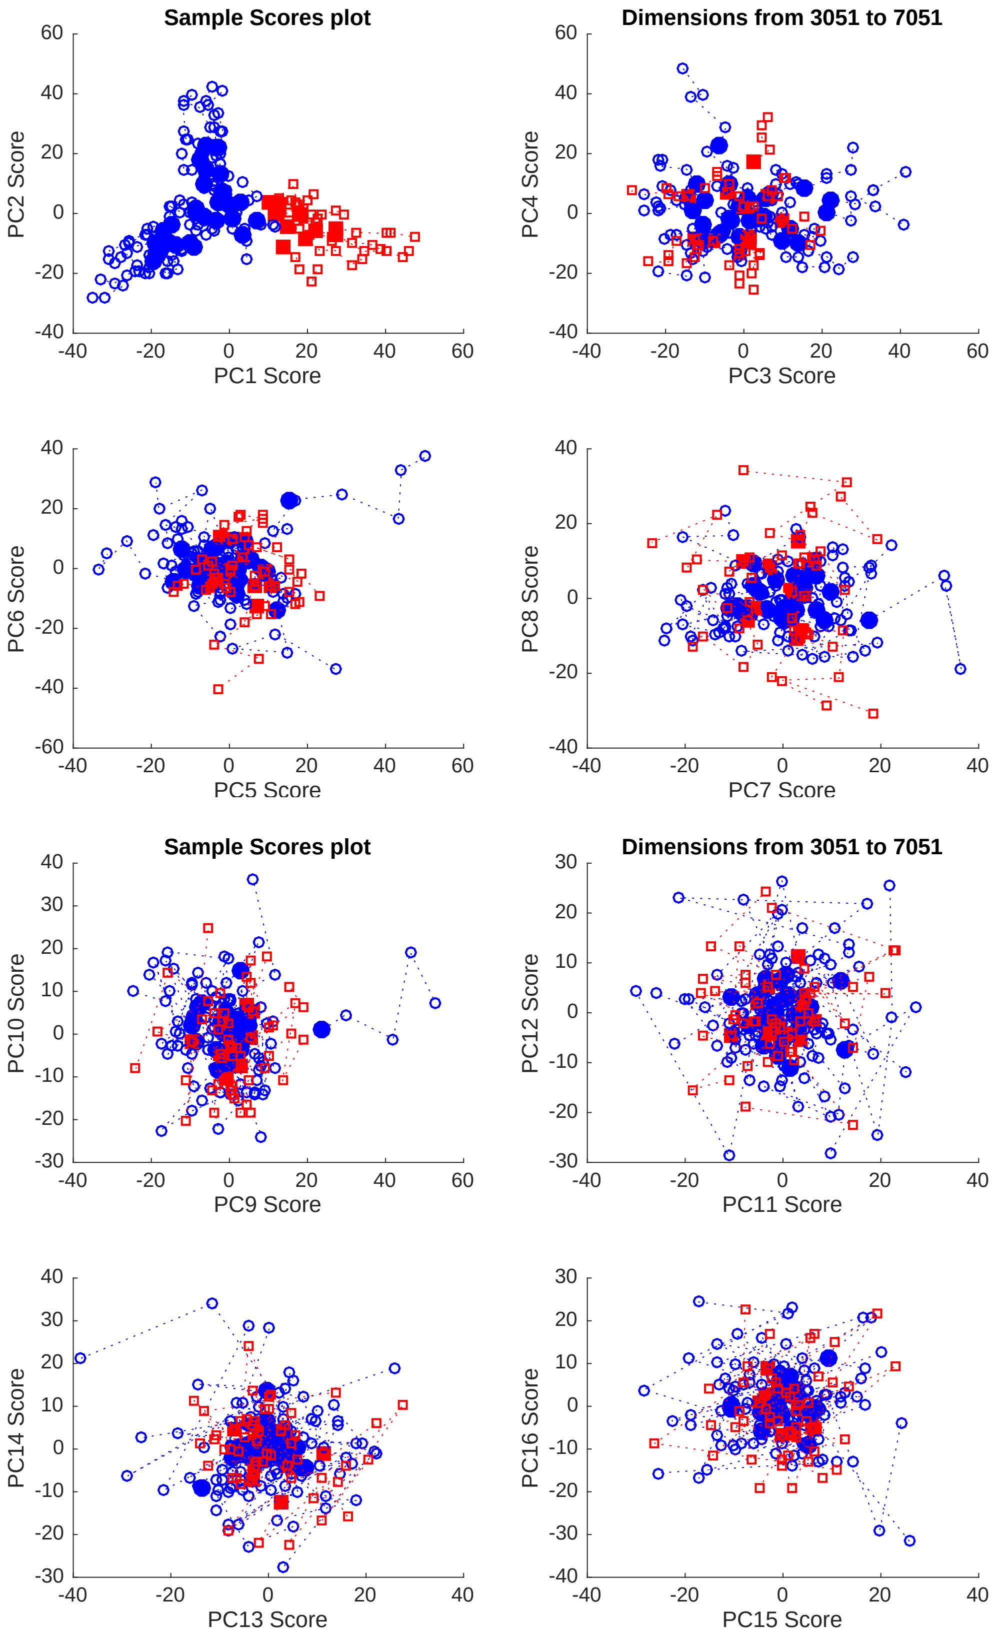


Fig. S9. Noise-augmented leukemia data. Scores for components 1–16. Filled symbols are scores from $\mathcal{X}_0$ and void symbols are from $\mathcal{X}_\ell$ ($\ell = 1, \ldots, 4$). The scores for the same patient are connected by line segments.

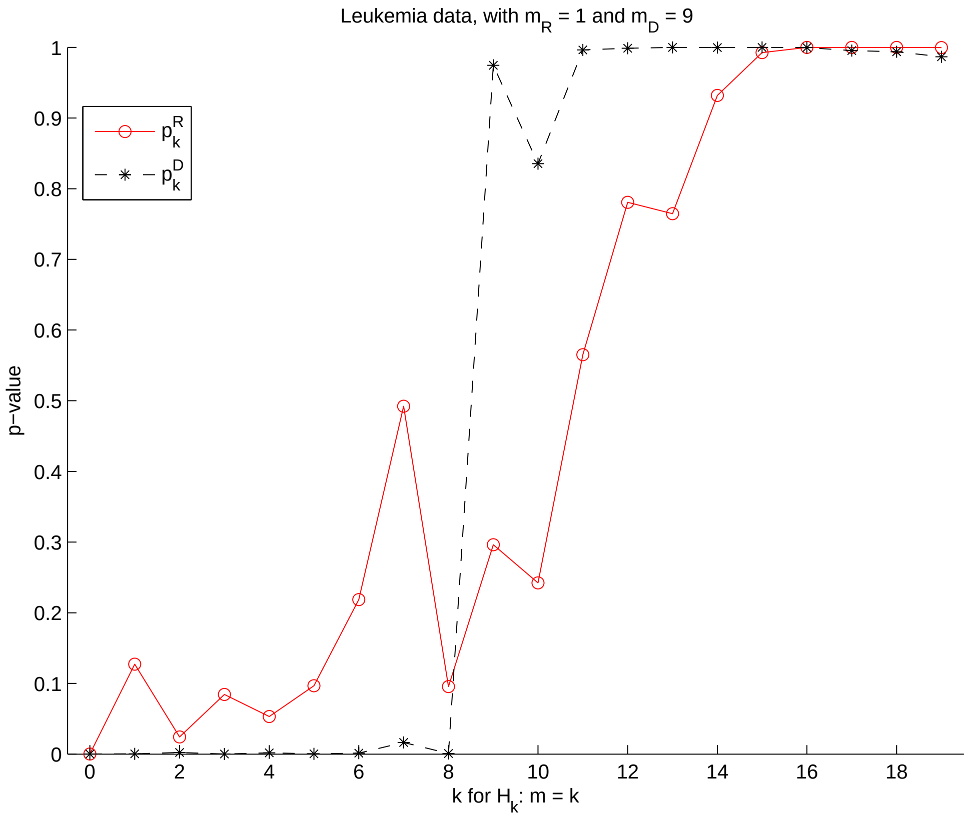


Fig. S10. The sequences of p-values $p_k^R$ and $p_k^D$ for the leukemia data.

PASSEMIER, D. & YAO, J. (2014). Estimation of the number of spikes, possibly equal, in the high-dimensional case. *J. Multivar. Anal.* **127**, 173–183.
